# Supplementary material for: Stripe order in the underdoped region of the two-dimensional Hubbard model
Source: arXiv:1701.00054 source file (2017-12-08)
Supplement: Supplementary file 1 [file supplementary.pdf]

# Supplementary Materials for "Stripe order in the underdoped region of the two-dimensional Hubbard model"

Bo-Xiao Zheng[1,2*†], Chia-Min Chung[3†], Philippe Corboz[4†], Georg Ehlers[5†], Ming-Pu Qin[6†], Reinhard M. Noack[5], Hao Shi[6†], Steven R. White[3], Shiwei Zhang[6], Garnet Kin-Lic Chan[1*]

[1]Division of Chemistry and Chemical Engineering, California Institute of Technology, Pasadena, CA 91125, USA
[2]Department of Chemistry, Princeton University, Princeton, NJ 08544, USA
[3]Department of Physics and Astronomy, University of California, Irvine, CA
[4]Institute for Theoretical Physics and Delta Institute for Theoretical Physics, University of Amsterdam, Science Park 904, 1098 XH Amsterdam, The Netherlands
[5]Fachbereich Physik, Philipps-Universität Marburg, 35032 Marburg, Germany
[6]Department of Physics, The College of William and Mary, Williamsburg, VA 23187, USA

*To whom correspondence should be addressed; E-mail: boxiao.zheng@gmail.com
*To whom correspondence should be addressed; E-mail: gkc1000@gmail.com
†These authors contributed equally to the calculations in this work.

## S1 Structure of the supplementary information

Section S2 contains notes on the figures and main discussion. Section S3 contains a summary of the best energy data used to compare the relative stripe energetics. Section S4 discusses the estimate of the long-range Coulomb effects. The remaining sections describe in detail the calculations performed using AFQMC, DMRG, hybrid DMRG, DMET, and iPEPS.

# S2 Additional information for figures and main discussion

Fig. 1: The plotted energies (units of $t$) correspond to the following specific calculations.

- AFQMC: $-0.766 \pm 0.001$ from extrapolation to $\infty$ (in both length and width directions) clusters with pinning fields.
- DMRG: $-0.7627 \pm 0.0005$ from extrapolation to $\infty \times 6$ clusters with pinning fields using the hybrid momentum/real-space representation (h-DMRG).
- DMET: $-0.77063 \pm 0.00001$ from $8 \times 2$ clusters with spin-flip boundary conditions.
- iPEPS: $-0.7673 \pm 0.002$ from $16 \times 2$ supercells with extrapolation to zero truncation error.

Note that the error bars only reflect errors that can be estimated from the calculations themselves, and not all systematic errors.

Discussion of Fig. 2: The metastable DMET state on the $\sqrt{5} \times 2$ lattice is slightly higher in energy than the ground-state. It is a "stripe-like" state, but appears to be frustrated at this unit-cell size. It is a little hard to estimate the relative energy of this state and the vertical striped ground state as the tilted impurity cluster energies are systematically shifted with respect to the energies of the non-tilted clusters. We estimate the relative energy of the $\sqrt{5} \times 2$ state as $E = E_{\sqrt{5}\times 2} - E_{\sqrt{2}\times 2} + E_{2\times 2}$, which includes the difference between the $2 \times 2$ cluster uniform $d$-wave state energy and tilted $\sqrt{2} \times 2$ cluster uniform $d$-wave state. This gives an estimate of $\sim 0.005t$ above the vertical striped state.

Fig. 3 and Fig. 6: The plotted energies are summarized in Section S3, Tables S1 to S4.

Fig. 4: The plotted orders correspond to the following specific calculations.

- DMET: from $8 \times 2$ calculations with spin-flip boundary condition. We plotted two unit-cells to illustrate the complete spin pattern.

- AFQMC: from $48 \times 4$ calculations with cylinder boundary conditions (periodic in the shorter direction). We duplicated the pattern in a $8 \times 2$ rectangle to illustrate the complete spin pattern.

- iPEPS: from the $8 \times 2$ calculations with 16 independent tensors. The numbers are shown for the largest bond dimension used. We plot the pattern in a $16 \times 2$ region to illustrate the complete spin pattern.

- DMRG: from a $32 \times 6$ calculation with cylinder boundary conditions. The results are extrapolated to zero truncation error. We duplicated the pattern in a $8 \times 2$ rectangle to illustrate the complete spin pattern.

Notes on Fig. 5(D): The plot is reproduced from part of Fig. S22. See the figure caption for detail.

Wavelengths of stripes: A key feature of the stripes that we see is that each stripe acts as an antiferromagnetic domain wall. As a well-known consequence, at $1/8$ doping for half-filled stripes, the wavelength associated with the AF periodicity $(8)$ is twice that of the charge periodicity $(4)$. As an oversimplified but useful characterization of this periodicity, we describe it by labeling the spin pattern along a fixed row, assuming the stripe is width $1$: $\ldots \cdot \uparrow\downarrow\uparrow \cdot \downarrow\uparrow\downarrow \cdot \uparrow\downarrow\uparrow \cdot \ldots$.Here the $\cdot$'s indicate the positions of the stripes, and the patterns $\uparrow \cdot \downarrow$ or $\downarrow \cdot \uparrow$ signify the domain wall nature of the stripe. Consider a charge wavelength which is an odd integer, e.g. $5$: $\ldots \cdot \uparrow\downarrow\uparrow\downarrow \cdot \uparrow\downarrow\uparrow\downarrow \ldots$ We see that the ratio of AF and charge wavelengths is one in this case, not two! This odd-even alternation is potentially confusing, particularly if one has non-integer charge periodicity.

However, experimentally, one looks at structure factors, noting peaks near $(\pi, \pi)$. The locations of the peaks nearest $(\pi, \pi)$ do not show any odd/even alternation. To see this note that the shift of the $k$-space origin to $(\pi, \pi)$, for one particular row, is equivalent to an alternating sign

chain $-1^x$ in the AF pattern, e.g. for charge wavelength $4$,

$$\ldots \cdot \uparrow\downarrow\uparrow \cdot \downarrow\uparrow\downarrow \cdot \uparrow\downarrow\uparrow \cdot \ldots \rightarrow \ldots \cdot \uparrow\uparrow\uparrow \cdot \downarrow\downarrow\downarrow \cdot \uparrow\uparrow\uparrow \cdot \ldots$$

and for charge wavelength $5$

$$\ldots \cdot \uparrow\downarrow\uparrow\downarrow \cdot \uparrow\downarrow\uparrow\downarrow \ldots \rightarrow \ldots \cdot \uparrow\uparrow\uparrow\uparrow \cdot \downarrow\downarrow\downarrow\downarrow \ldots$$

In both the even and odd cases, the distance of peaks from $(\pi, \pi)$ corresponds to an AF "wavelength" of twice the charge wavelength.

# S3 Summary of stripe energy results

Table S1: Best estimates of energy (per site) of stripes and competing states for $U/t = 8$. AFQMC numbers obtained as described in section S5, DMRG numbers obtained as described in section S6, Hybrid (h-) DMRG numbers obtained as described in section S7, iPEPS numbers obtained as described in section S8, DMET numbers obtained as described in section S9. For the AFQMC calculations (PBC) denotes periodic boundary conditions used on both the short- and long-axes of the cylinder. For the DMRG (real-space) calculations, periodic boundary conditions were used along the short axis, open boundary conditions on the long axis. For the h-DMRG calculations, periodic or anti-periodic boundary conditions were used on the short axis, denoted PBC or APBC. SF denotes that the DMET correlation potential in the spin-channel is flipped, doubling the spin wavelength. (Thus the $8 \times 2$ (SF) pattern in DMET has a charge wavelength of 8 but a spin wavelength of 16.)

| Method | Size | Wavelength | Energy ($t$) | Error ($t$) |
|---|---|---|---|---|
| AFQMC | $12 \times 8$ (PBC) | 6 | $-0.7653$ | 0.0002 |
| AFQMC | $14 \times 8$ (PBC) | 7 | $-0.7653$ | 0.0002 |
| AFQMC | $16 \times 8$ (PBC) | 8 | $-0.7668$ | 0.0002 |
| AFQMC | $18 \times 8$ (PBC) | 9 | $-0.7655$ | 0.0002 |
| AFQMC | $20 \times 8$ (PBC) | 10 | $-0.7653$ | 0.0002 |
| AFQMC | $\infty \times 4$ | 8 | $-0.7680$ | 0.0001 |
| AFQMC | $\infty \times 6$ | 8 | $-0.7653$ | 0.0003 |
| AFQMC | $\infty \times 8$ | 8 | $-0.7656$ | 0.0004 |
| DMRG | $\infty \times 4$ | 8 | $-0.76598$ | 0.00003 |
| DMRG | $\infty \times 6$ | 5 | $-0.7615$ | 0.0004 |
| DMRG | $\infty \times 6$ | 8 | $-0.762$ | 0.001 |
| DMRG | $\infty \times 7$ | 7 | $-0.762$ | 0.001 |
| DMRG | $\infty \times 6$ | 9 | $-0.751$ | 0.0016 |
| h-DMRG | $\infty \times 6$ (PBC) | 5 | $-0.76210$ | 0.00005 |
| h-DMRG | $\infty \times 4$ (APBC) | 8 | $-0.76057$ | 0.00007 |
| h-DMRG | $\infty \times 4$ (PBC) | 8 | $-0.7657$ | 0.0003 |
| h-DMRG | $\infty \times 4$ (av.)[a] | 8 | $-0.7631$ | 0.0003 |
| h-DMRG | $\infty \times 6$ (PBC) | 8 | $-0.7627$ | 0.0005 |
| iPEPS | $2 \times 2$[b] | 2 | $-0.7560$ | 0.0025 |
| iPEPS | $5 \times 2$ | 5 | $-0.7632$ | 0.0018 |
| iPEPS | $7 \times 2$ | 7 | $-0.7629$ | 0.0026 |
| iPEPS | $16 \times 2$ | 8 | $-0.7673$ | 0.002 |

[a] Average of APBC and PBC results.
[b] Using 2 independent tensors.

| Method | Size | Wavelength | Energy ($t$) | Error ($t$) |
|---|---|---|---|---|
| iPEPS | $16 \times 16$[c] | diag. $4\sqrt{2}$ | $-0.7581$ | $0.0014$ |
| DMET | $2 \times 2$ | $d$-wave | $-0.7580$ | $0.0005$ |
| DMET | $3 \times 2$ | $3$ | $-0.7437$ | $0.0009$ |
| DMET | $4 \times 2$ (SF) | $4$ | $-0.7614$ | $0.00005$ |
| DMET | $5 \times 2$ | $5$ | $-0.7691$ | $0.001$ |
| DMET | $6 \times 2$ (SF) | $6$ | $-0.7706$ | $0.00007$ |
| DMET | $7 \times 2$ | $7$ | $-0.7704$ | $0.0003$ |
| DMET | $8 \times 2$ (SF) | $8$ | $-0.7706$ | $0.00001$ |
| DMET | $9 \times 2$ | $9$ | $-0.7658$ | $0.0008$ |
| DMET | $2\sqrt{2} \times \sqrt{2}$ | $d$-wave | $-0.7620$ | $0.00001$ |
| DMET | $5\sqrt{2} \times \sqrt{2}$ | frustrated[d] | $-0.7689$ | $0.0008$ |

Table S2: Energy (per site) of stripes with UHF using effective $U/t = 2.7$. The effective $U$ is determined by self-consistent AFQMC procedure, described in Section S5.

| Size | Wavelength | Energy ($t$) | Error ($t$) |
|---|---|---|---|
| $8 \times 2$ (TABC) | $4$ | $-1.0912$ | 0.0004 |
| $10 \times 2$ (TABC) | $5$ | $-1.0930$ | 0.0003 |
| $12 \times 2$ (TABC) | $6$ | $-1.0944$ | 0.0002 |
| $14 \times 2$ (TABC) | $7$ | $-1.0979$ | 0.0003 |
| $16 \times 2$ (TABC) | $8$ | $-1.1004$ | 0.0002 |
| $18 \times 2$ (TABC) | $9$ | $-1.0993$ | 0.0001 |
| $20 \times 2$ (TABC) | $10$ | $-1.0984$ | 0.0002 |
| $22 \times 2$ (TABC) | $11$ | $-1.0974$ | 0.0002 |

[c] Using 16 independent tensors.
[d] No clear pattern, order appears to be frustrated.

Table S3: Best estimates of energy (per site) of stripes and competing states for $U/t = 6$. AFQMC numbers obtained as described in section S5, DMET numbers obtained as described in section S9. Other details as above.

| Method | Size | Wavelength | Energy ($t$) | Error ($t$) |
|---|---|---|---|---|
| AFQMC | $12 \times 8$ (PBC) | 6 | $-0.8684$ | 0.0001 |
| AFQMC | $14 \times 8$ (PBC) | 7 | $-0.8692$ | 0.0001 |
| AFQMC | $16 \times 8$ (PBC) | 8 | $-0.8718$ | 0.0001 |
| AFQMC | $18 \times 8$ (PBC) | 9 | $-0.8701$ | 0.0001 |
| AFQMC | $20 \times 8$ (PBC) | 10 | $-0.8702$ | 0.0001 |
| DMET | $2 \times 2$ | $d$-wave | $-0.8679$ | 0.0007 |
| DMET | $3 \times 2$ | 3 | $-0.85867$ | 0.00004 |
| DMET | $4 \times 2$ | 4 | $-0.85890$ | 0.00004 |
| DMET | $5 \times 2$ | 5 | $-0.86836$ | 0.00001 |
| DMET | $6 \times 2$ (SF) | 6 | $-0.87247$ | 0.00001 |
| DMET | $7 \times 2$ | 7 | $-0.87363$ | 0.00002 |
| DMET | $8 \times 2$ (SF) | 8 | $-0.87667$ | 0.0007 |

Table S4: Best estimates of energy (per site) of stripes and competing states for $U/t = 12$. AFQMC numbers with twist averaged boundary conditions (TABC) obtained as described in section S5, DMET numbers obtained as described in section S9, DMRG numbers obtained as described in section S6. Other details as above.

| Method | Size | Wavelength | Energy ($t$) | Error ($t$) |
|---|---|---|---|---|
| AFQMC | $10 \times 8$ (TABC) | 5 | $-0.6446$ | 0.0006 |
| AFQMC | $12 \times 8$ (TABC) | 6 | $-0.6452$ | 0.0004 |
| AFQMC | $14 \times 8$ (TABC) | 7 | $-0.6461$ | 0.0006 |
| AFQMC | $16 \times 8$ (TABC) | 8 | $-0.6458$ | 0.0006 |
| AFQMC | $18 \times 8$ (TABC) | 9 | $-0.6462$ | 0.0006 |
| AFQMC | $20 \times 8$ (TABC) | 10 | $-0.6450$ | 0.0006 |
| DMET | $2 \times 2$ | $d$-wave | $-0.63940$ | $0.00001$ |
| DMET | $4 \times 2$ (SF) | 4 | $-0.6505$ | $0.0001$ |
| DMET | $5 \times 2$ | 5 | $-0.6531$ | $0.0001$ |
| DMET | $6 \times 2$ (SF) | 6 | $-0.6526$ | $0.0002$ |
| DMET | $8 \times 2$ (SF) | 8 | $-0.6514$ | $0.0001$ |
| DMRG | $\infty \times 4$ | 4 | -0.641379 | 0.000052 |
| DMRG | $\infty \times 4$ | 5 | -0.64269 | 0.00019 |
| DMRG | $\infty \times 4$ | 6 | -0.64285 | 0.00021 |
| DMRG | $\infty \times 4$ | 8 | 0.64168 | 0.00023 |
| DMRG | $\infty \times 6$ | 4 | -0.6383 | 0.0026 |
| DMRG | $\infty \times 6$ | 5 | -0.64148 | 0.00059 |
| DMRG | $\infty \times 6$ | 6 | -0.6418 | 0.0013 |
| DMRG | $\infty \times 6$ | 8 | -0.6438 | 0.0019 |

## S4 Long-range Coulomb interaction

We estimate the long-range Coulomb interaction in the vertical stripes by computing the electrostatic potential energy from charge patterns obtained from the DMET calculations

$$e_{\text{Coul}} = \frac{1}{N_c} \sum_{i \in \text{imp}, j, i \neq j} (h_i - \bar{h})(h_j - \bar{h}) / 4\pi\varepsilon_0 \varepsilon r_{ij} \tag{S1}$$

where $N_c$ is the number of impurity sites, $h_i$ is the hole density on site $i$, and $\bar{h}$ is the average

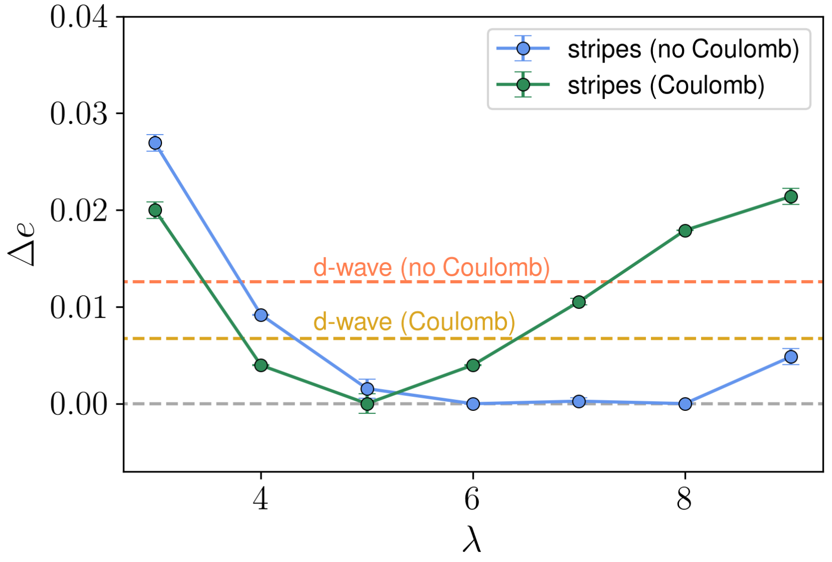


Figure S1: Energy landscape before and after adding the estimated long-range Coulomb interaction for vertical stripes of different wavelength. The charge distributions are from DMET calculations.

hole density (1/8). In atomic units, i.e. if we express the energy in Hartrees, and distance in Bohr, $1/4\pi\varepsilon_0 = 1$. The appropriate dielectric constant to use in a statically screened Coulomb interaction in the $CuO_2$ plane has been estimated to lie between about 4 and 27 (*50, 51*). We use a dielectric constant of $\varepsilon = 15.5$, and a lattice constant $a = 3.78$Å$= 7.14$ Bohr corresponding to the lattice constant of $La_2CuO_4$. We transform the computed Coulomb energy (per site) to units of $t$, using $t \sim 3000K \sim 0.01$ Hartree.

In 2D, the Coulomb summation converges reasonably fast. We choose a cutoff radius as 300 lattice spacings and converge the Coulomb energy to the fourth digit in units of $t$. The results for the DMET vertical stripes are shown in Fig. S1. The long-range Coulomb interaction favors shorter wavelength stripes and the homogeneous $d$-wave state, shifting the ground state to wavelength $5$ and making the uniform $d$-wave state also more competitive. Of course the above treatment of the Coulomb term is quite crude, neglects the effect of relaxation in the presence of the Coulomb interaction, and there is significant uncertainty in the dielectric. Nevertheless, the calculation provides an energy scale, $O(0.01t)$, over which the long-range Coulomb interaction is important.

# S5 AFQMC calculations

## S5.1 Details of the AFQMC calculations

We studied cylinders of dimension $l_y \times l_x$ ($l_x > l_y$) with several different boundary conditions. In the first set of calculations, which allow for direct comparison with the finite system DMRG calculations, we used open boundary conditions (OBC) along the $x$ direction and periodic boundary conditions (PBC) along the $y$ direction. We also applied pinning fields to pin the underlying spin structures. Several types of pinning fields were used depending on the targeted structure, as shown in Fig. S2. Along each edge, the pinning fields were always antiferromagnetic. With FM (AFM) pinning fields, we targeted an odd (even) number of nodes ($\pi$ phase shifts) in the system ($l_x$ is always even in our calculations). In some cases, we also applied pinning fields only on one edge to accommodate states with different wavelengths. The strength of the pinning fields is $|h| = 0.5$ (units of $t$) for all calculations. All these calculations used constrained path AFQMC method with self-consistent optimized trial wavefunctions (*33*).

In the second set of calculations, we used PBC along both directions, or twist averaged boundary conditions (TABC) along both directions. The twist averaging allows us to reduce the finite size errors in the total energy. These calculations used an unrestricted Hartree-Fock (UHF) trial wavefunction generated by an effective $U$. In the following, DMRG results shown for comparison are from section S6. Results are for $U = 8$ unless otherwise stated.

## S5.2 Wavelength 8 striped ground-state

The spin and hole structure of the $4 \times 16$, $6 \times 16$, $4 \times 24$, and $6 \times 32$ systems are plotted in Figs. S3, S4, S5, and S6 respectively. All the results are obtained with the self-consistent AFQMC method starting from free electron trial wavefunctions.

Exhaustive comparisons were made between AFQMC and DMRG in these systems. The ground state energies for these systems are listed in Table S5. The systematic error compared

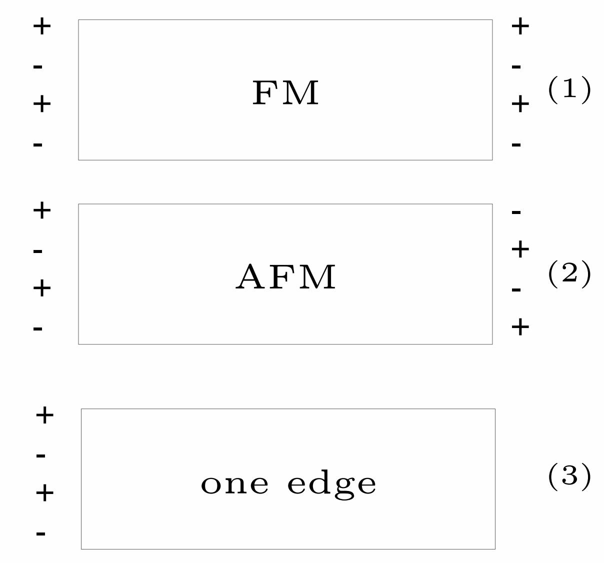


Figure S2: Different types of pinning fields. The relative phase between the pinning fields on the two edges is positive in (1) and negative in (2). We denote (1) and (2) by FM and AFM pinning fields respectively. In some cases, to accommodate states with different wavelengths, we also apply pinning fields on only one edge. We also studied systems with PBC and TABC along both edges, to reduce the finite size effects. Notice that the pinning field along each edge is always anti-ferromagnetic.

with DMRG from the constraint in AFQMC is about $-0.4\%$.

For the $6\times16$ system, two different pinning fields, i.e., AFM and FM, were tried. The energy with AFM pinning field (wavelength 8) is lower. For the $6\times32$ system, self-consistent AFQMC finds a ground state structure with wavelength $8$ ($4$ nodes) from a free electron trial wavefunction. We can also construct trial wavefunctions from the density obtained by DMRG. We calculated the energy using the two different trial wavefunctions constructed from the DMRG density for the two states ($4$ and $6$ nodes). The energy comparison of the two stripe states is shown in Table S5. We also did an AFQMC calculation by setting the trial wavefunction as an equal linear combination of the two trial wavefunctions. The state with wavelength $8$ survives after convergence. The energy difference between the two states is $\sim 0.001$ in DMRG and $\sim 0.003$ in AFQMC. Again the AFQMC energies are slightly lower than the DMRG energies due to the

Table S5: Ground state energies for different systems with pinning fields. DMRG results from section S6.

| Size | pinning field | state | DMRG | AFQMC |
|---|---|---|---|---|
| $4 \times 16$ | AFM | 2 nodes / wavelength $8$ | -0.77127(2) | -0.7744(1) |
| $6 \times 16$ (meta-stable) | FM | 3 nodes | -0.7682(3) | -0.7692(1) |
| $6 \times 16$ | AFM | 2 nodes / wavelength $8$ | -0.7691(5) | -0.7725(2) |
| $4 \times 24$ | FM | 3 nodes / wavelength $8$ | -0.76939(3) | -0.7727(2) |
| $6 \times 32$ (meta-stable) | AFM | 6 nodes | -0.7648(3) | -0.7663(1) |
| $6 \times 32$ | AFM | 4 nodes / wavelength $8$ | -0.7658(7) | -0.7691(2) |

constrained path approximation. However, the results are consistent (the state with wavelength $8$ has lower energy).

After convergence, for all the systems studied, the effective $U$ in the self-consistent AFQMC calculation is about $U = 2.7$.

## S5.3 Comparison of different wavelengths

### S5.3.1 $4 \times 40$

We studied the $4 \times 40$ cylinder which accommodates the states with wavelengths of 5 and 8. We used different pinning fields to favor states with different wavelengths.

We applied AFM pinning fields to favor states with an even number of nodes, that is states with wavelengths of $5$, $10$ or $20$. The result from the self-consistent AFQMC with a free trial wavefunction is a state with wavelength $10$. If we used a trial wavefunction with wavelength

Table S6: Ground state energies of $4 \times 40$ system. Pinning fields are applied on only one edge. The energies for the two states with wavelength $8$ and $10$ are very close, however, when we carry out the AFQMC calculation using the equal linear combination of the two trial wavefunctions as the initial wavefunction, the state with wavelength $8$ survives.

| pinning field | state | AFQMC |
|---|---|---|
| One edge | 8 nodes / wavelength $5$ (doesn't survive in self-consistent AFQMC) | $-0.7657(2)$ |
| One edge | 5 nodes / wavelength $8$ | $-0.7663(1)$ |
| One edge | 4 nodes / wavelength $10$ | $-0.7665(3)$ |

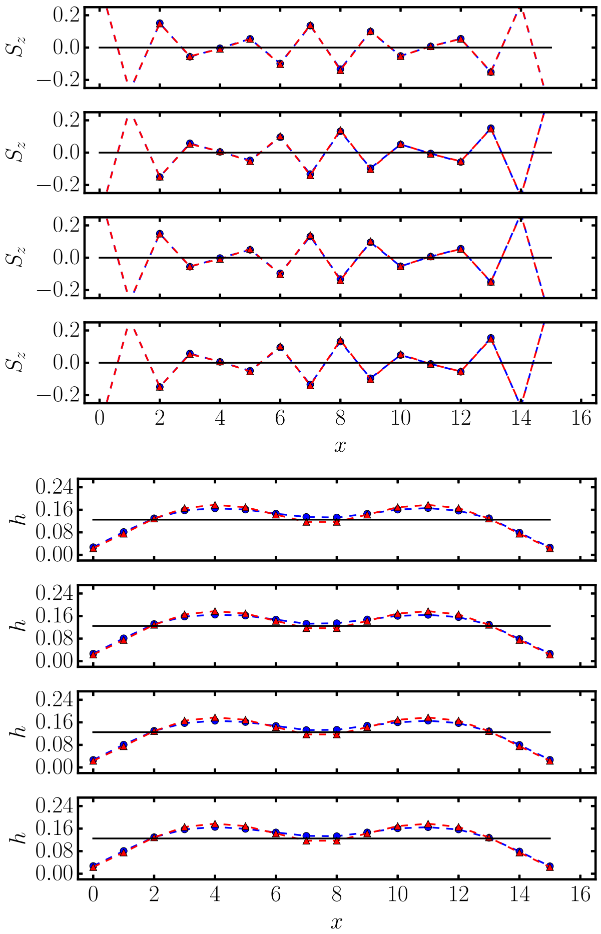

Figure S3: Spin and hole densities along $l_x$ (with each panel for one value of $l_y$) in $4 \times 16$ system with AFM pinning fields. Blue circles are for AFQMC and red triangles are for DMRG.

5 (*52*) to start the self-consistent AFQMC, the final pattern again converged to wavelength 10. This suggests the stripe with wavelength 5 is a higher energy state. The spin and charge patterns are plotted in Fig. S7.

We also tried FM pinning fields with which we obtain the ground state with wavelength 8. The spin and charge pattern are plotted in Fig. S8.

To compare the patterns with wavelength 8 and wavelength 10, we studied the $4 \times 40$ system with pinning fields on only left edge of the cylinder which accommodates both patterns. We find that the energies for these two trial wavefunctions are very close: $-0.7665(3)$ for wavelength 10

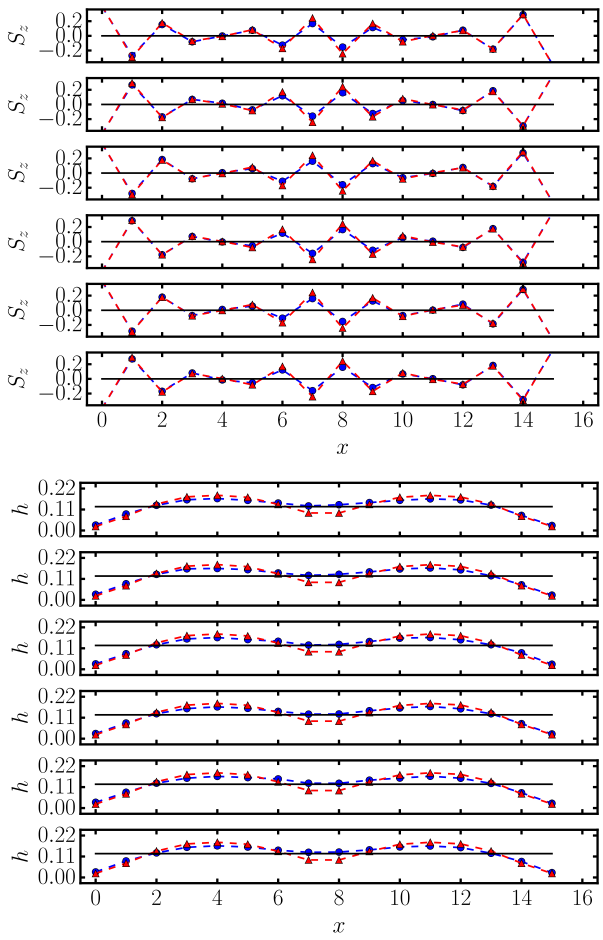


Figure S4: $6 \times 16$, with AFM pinning fields. Blue circles are for AFQMC and red triangles are for DMRG.

and $-0.7663(1)$ for wavelength 8. However, if we use an equal linear combination of the two as the initial wavefunction, the pattern with wavelength 8 survives in the AFQMC calculation. This suggests that the pattern with wavelength 8 is the true ground state. We also calculated the energy of this system using the unstable state with wavelength $5$ as the trial wavefunction. The energy is higher: $-0.7657(2)$.

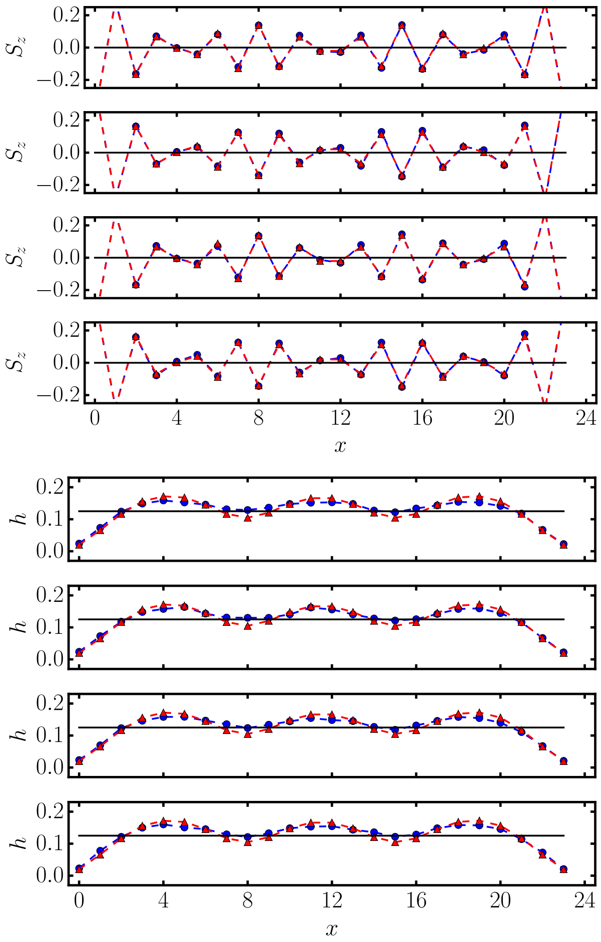


Figure S5: $4 \times 24$, with FM pinning fields. Blue circles are for AFQMC and red triangles are for DMRG.

### S5.3.2 $4 \times 48$

We studied the $4 \times 48$ cylinder which accommodates states with wavelengths of $6$ and $8$. Unlike the $4 \times 40$ case, the AFM pinning fields are compatible with both patterns.

From a trial wavefunction with wavelength $8$, the self-consistent result is plotted in Fig. S9. The converged state has wavelength of 12 with energy $-0.7701(1)$.

The self-consistent result from a free trial wavefunction is plotted in Fig. S10. The converged energy is $-0.7699(1)$.

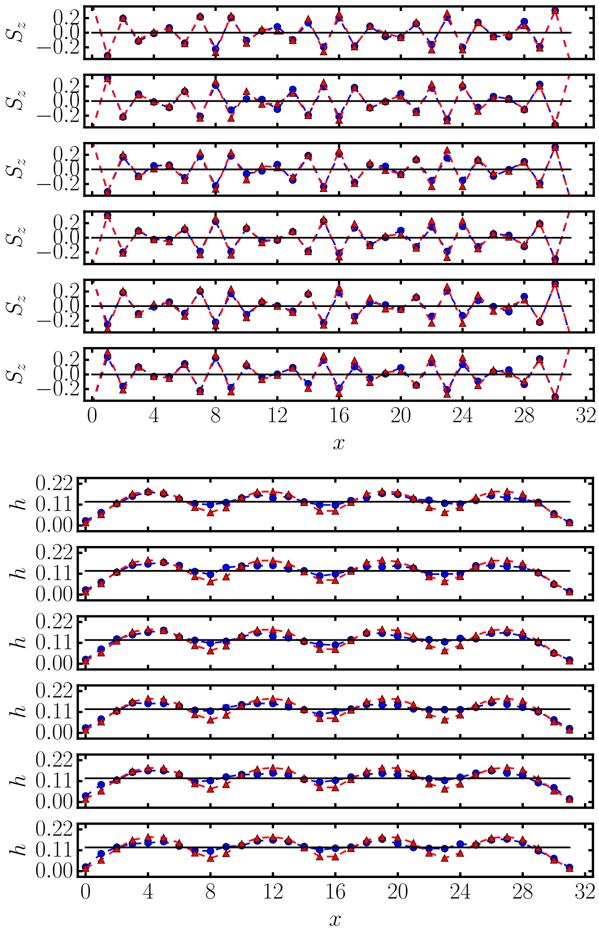


Figure S6: $6 \times 32$, with AFM pinning fields. Blue circles are for AFQMC and red triangles are for DMRG.

As in the $4 \times 40$ case, to compare the two states, we can carry out an AFQMC calculation using an equal linear combination of the two converged trial wavefunctions as a trial wavefunction. After a step of the self-consistent AFQMC calculation, the state with wavelength $8$ survives, which indicate, that this state is the true ground state.

We can also construct a trial wavefunction with wavelength $6$ (*52*). With the self-consistent AFQMC calculation this pattern does not survive, but turns into one with wavelength $8$ after convergence. For the first few steps when the pattern still has wavelength $6$, the energy is $-0.7693(1)$, which is higher than the energies of wavelength $8$ and $12$.

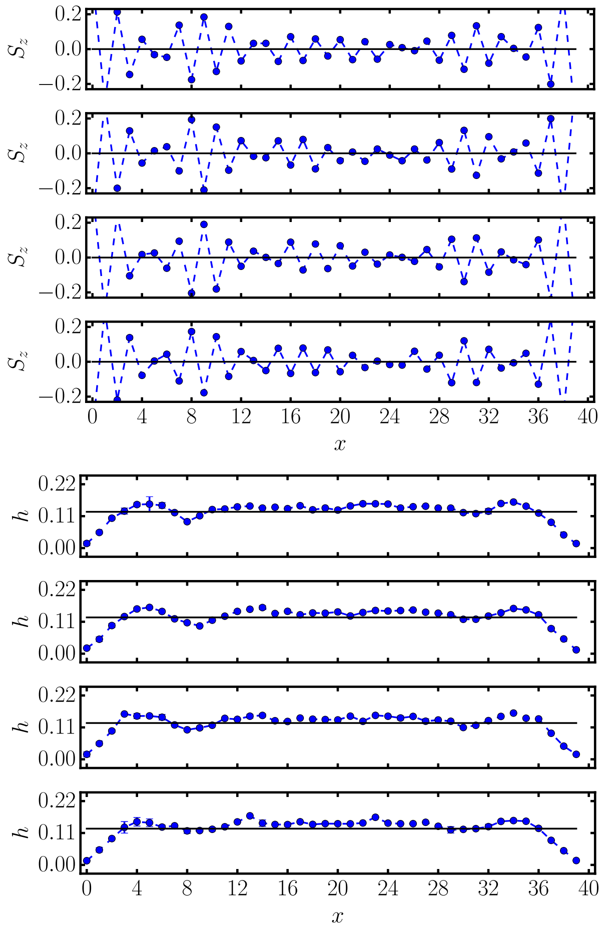

Figure S7: $4 \times 40$, with AFM pinning fields. Each panel is for one value of $l_y$.

#### S5.3.3 $U = 6$ and $U = 12$ cases

We also compared the states with wavelength $7, 9$ with $8$ using $4 \times 56$ and $4 \times 72$ cells for $U = 6$, and wavelength $6$ with $8$ using a $4 \times 48$ cell for $U = 12$. For $U = 6$, even though the energies for states with wavelength $7, 8$ and $9$ are close, the state with wavelength $8$ is more robust in the self-consistent AFQMC calculation. For $U = 12$, the energies of states with wavelength $6$ and $8$ are essentially indistinguishable. We carried out calculations using as a trial wave-function an equal linear combination of two trial wave-functions optimized for the two wavelengths. After one step of the self-consistent AFQMC calculation, the state with wavelength $8$ survives. This

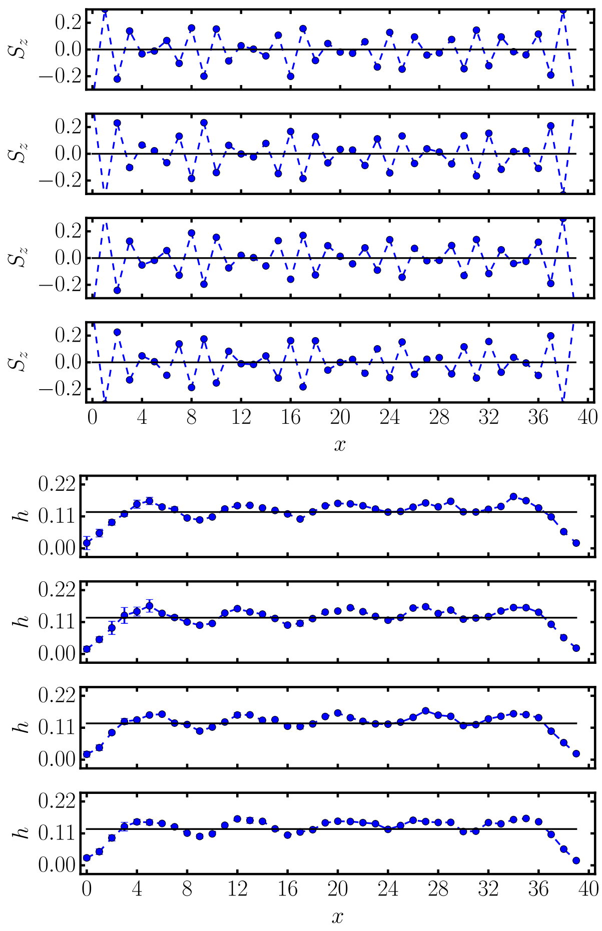

Figure S8: $4 \times 40$, with FM pinning fields. Each panel is for one value of $l_y$.

suggests that the state with wavelength 8 is the ground state, which is consistent with the result of the fit of the E vs $\lambda$ curve, in which $\lambda = 8$ is the minimum.

## S5.4 Comparing states using PBC and TABC

From calculations on cylinders in the previous sections, we can estimate an effective renormalized $U$ for $U = 8$, $1/8$ doping to be around $U = 2.7$ (for PBC, we would expect the effective $U$ to be slightly larger). In this section, we first compare the UHF energies at $U = 2.7$ for different wavelengths which are shown in the left panel of Fig. S11. Both PBC and TABC are used. With TABC, the finite size effects can be reduced. We use different sizes ($8 \times 2\lambda$) to target states with

Table S7: Ground state energies of the $4 \times 48$ system. AFM pinning fields are applied. The energies for the two stable patterns are very close. However, when we carry out the AFQMC calculation using the equal linear combination of the two trial wavefunctions as the initial wavefunction, the state with wavelength $8$ survives.

| pinning field | state | AFQMC |
|---|---|---|
| AFM | $8$ nodes / wavelength $6$ (doesn't survive in self-consistent AFQMC) | $-0.7693(1)$ |
| AFM | $6$ nodes / wavelength $8$ | $-0.7701(1)$ |
| AFM | $4$ nodes / wavelength $12$ | $-0.7699(1)$ |

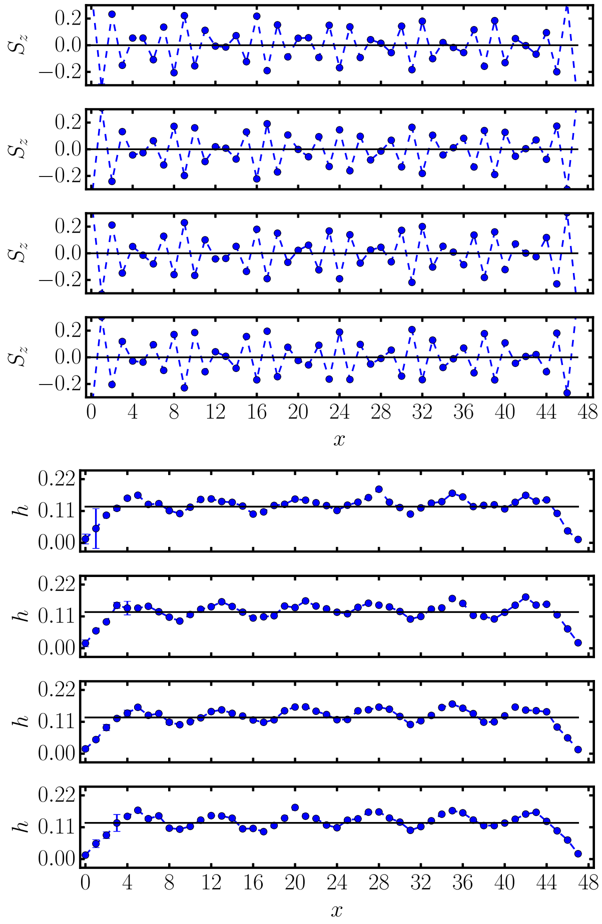


Figure S9: Wavelength $= 8$ state. $4 \times 48$, with AFM pinning fields. A trial wavefunction with wavelength $8$ is used in the first step of the self-consistent AFQMC calculation. Each panel is for one value of $l_y$.

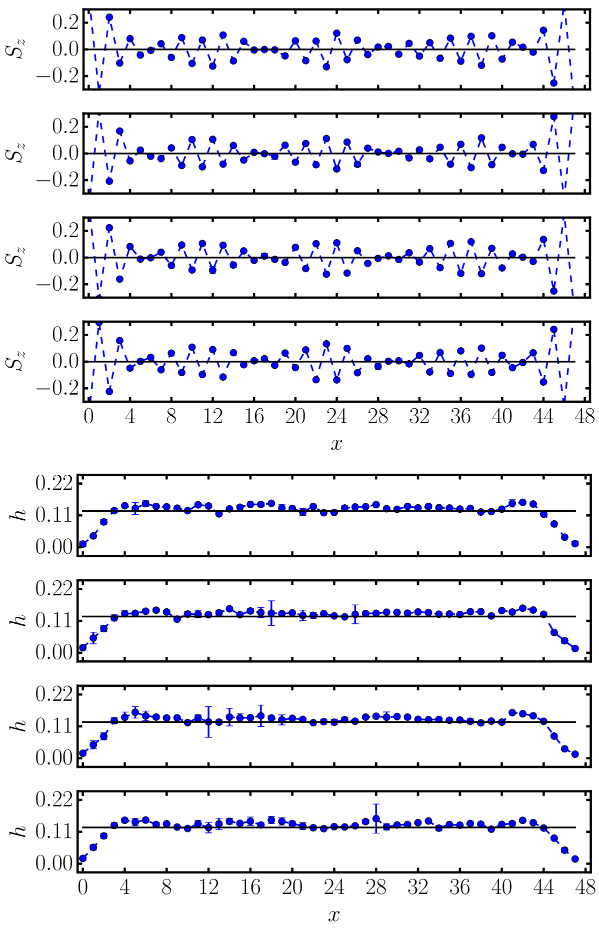


Figure S10: Wavelength $= 12$ state. $4 \times 48$, with AFM pinning fields. Free electron trial wavefunction is used in the first step of the self-consistent AFQMC calculation. Each panel is for one value of $l_y$.

different wavelengths ($\lambda$). We can find a minimum at wavelength $8$ for both PBC and TABC energies.

Next, we use the UHF wavefunctions with $U = 2.7$ as trial wavefunctions in the AFQMC calculations at $U = 8$, using supercells with the same size. The results are plotted in the right panel of Fig. S11. For PBC energies, there is a minimum at wavelength $8$. For TABC, the energies for wavelength $7, 8, 9$ are very close.

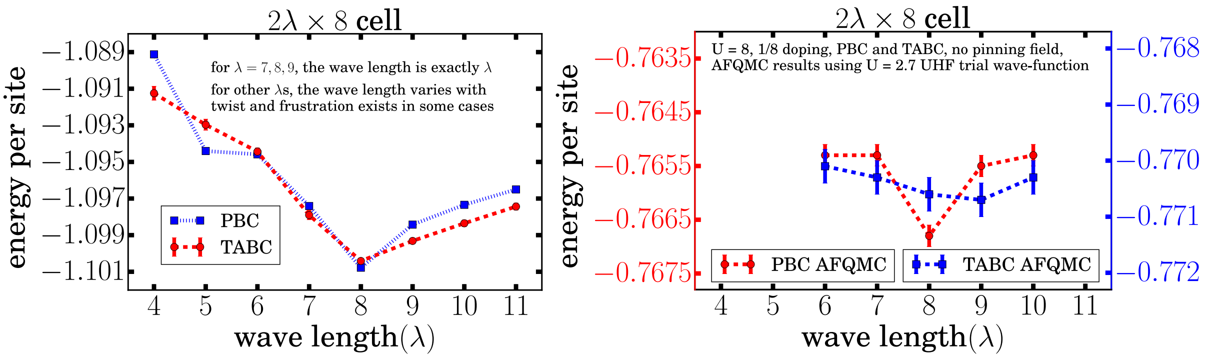


Figure S11: Left: UHF energy with effective $U = 2.7$. Right: AFQMC energy of $U = 8$ using the UHF trial wavefunction in the left panel.The TABC value for wavelength 8, computed here with an UHF trial wavefunction with $U_{eff} = 2.7$, is consistent with that from a free-electron trial wavefunction (*53*). Using a generalized Hartree-Fock (GHF) trial wavefunction gives a slightly improved result of -0.766(1) (*24*).

## S5.5 Energy of wavelength 8 state at U = 8 in the thermodynamic limit

To remove the finite-size effects in the computed ground-state energy for the state with wavelength $8$, we extrapolated the energies for systems with length, $16, 32, 48$, and $64$, and width, $4, 6$, and $8$. In Fig. S12 it is seen that the energies are indistinguishable for width, $6$ and $8$ which means the energy is converged to the targeted statistical accuracy with width $6$. We also confirmed the width convergence with length $32$ systems. The energies are $-0.7691(2)$, $-0.7688(2)$, $-0.7691(2)$, and $-0.7694(3)$ for width $6, 8, 10$, and $12$ systems respectively.

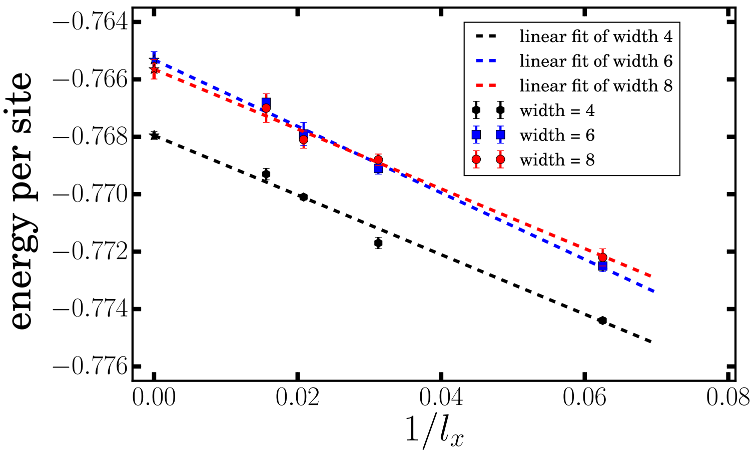


Figure S12: Energies for wavelength 8 state of various lengths and widths for $U = 8$. AFM pinning fields are applied. Linear fits of $1/l_x$ are shown. The infinite length values and error bars from extrapolation are marked as stars in the plot.

# S6 Lattice-basis DMRG

## S6.1 Details of the lattice-basis DMRG calculations

We considered cylinders of size $L_x \times L_y$ with $L_x > L_y$, an open boundary in the $x$ direction and a periodic boundary in the $y$ direction. We first considered systems with fixed particle number at $(1/8$ doping, and compared the energies of stripe states with different wavelengths.

To stabilize the states with particular wavelengths, we used as initial states product states with holes in the desired locations, and applied temporary fields and chemical potentials on the whole system in the first few sweeps. A temporary chemical potential of strength $2.0$ is applied on the sites where the holes are supposed to be in the final striped state, and a temporary magnetic field of strength $0.5$ is applied to fit the anti-ferromagnetic domains between holes. After the first few sweeps (typically up to bond dimension $m = 600$) the temporary field and chemical potential is turned off, and the state is called "stable" in the DMRG simulation if it keeps the same features (same wavelength in our case). In some cases, a pinning field of strength $|h| = 0.5$ at the edges is kept in the full simulation to further stabilize the state, but this does not change the total energy in the extrapolation to infinite length.

We next considered pairing order. To measure the pairing order, we simulated in grand canonical ensemble i.e. without total particle number conservation. The chemical potentials were tuned so that the expectation value of the particle number is close to the desired value ($7/8$ of the number of sites). We applied pairing fields at the edges, to break total particle number conservation, and observed how the pairing order decays into the bulk.

## S6.2 U=8, Fixed particle number

### S6.2.1 Energy

We summarize the energies of different stripe states on infinite-length cylinders in TableS8. The states of wavelength $7 \sim 8$ have the lowest energies, and the state of wavelength $5$ has a slightly

| size | wavelength | energy |
|---|---|---|
| $\infty \times 4$ | 8 | $-0.76598(3)$ |
| $\infty \times 6$ | 5 | $-0.7615(4)$ |
| $\infty \times 6$ | 8 | $-0.762(1)$ |
| $\infty \times 7$ | 7 | $-0.762(1)$ |
| $\infty \times 6$ | 9 | $-0.751(16)$ |

Table S8: Energies of different stripe states for $U = 8$ with different wavelengths on infinite-length cylinders.

higher energy. The state of wavelength $9$ is unstable, with a much higher energy.

#### S6.2.2 Width-4 cylinders

The cylinder sizes $8 \times 4$, $16 \times 4$, and $24 \times 4$ were considered. The ground state on width-4 cylinders was found to have wavelength $8$, each stripe contains $4$ holes (see Fig. S13). To stabilize the state and improve the convergence, we applied magnetic pinning fields on the edges; however the states without pinning fields were first calculated and had the same wavelengths. The pinning field was chosen to fit the anti-ferromagnetic pattern at the edges, with the strength $|h| = 0.5$. Fig.S13 shows the spin and hole density expectation values for a $24 \times 4$ cylinder. The energy extrapolation to infinite length is shown in Fig.S14.

#### S6.2.3 Width-6 cylinders, wavelengths $5$ and $8$

Cylinder sizes of $16 \times 6$, $32 \times 6$ and $48 \times 6$ were considered. In the width-6 cylinders we found competing states with close energies for wavelengths $5$ and $8$. For wavelength-$5$ state, each stripe contains $4$ hole, and for wavelength-$8$ state, each stripe contains $6$ holes. See Fig.S17 for the spin and hole densities of the two states. We found that the wavelength $8$ state has a lower energy. Note that for a fixed bond dimension and a fixed system size, the energy of wavelength $5$ is typically lower than the energy of wavelength $8$, and a DMRG simulation with a random initial state will end up finding the wavelength $5$ state. The fact that the wavelength $8$ state has

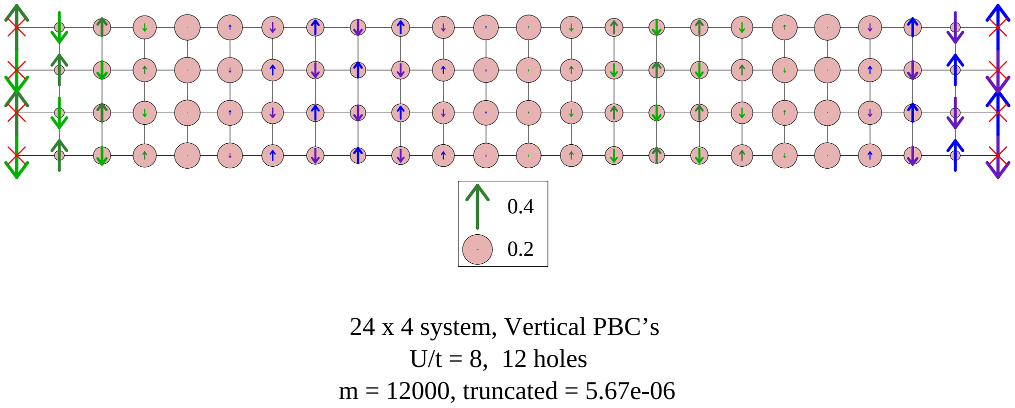


Figure S13: Spin (arrow) and hole density (circle) expectation values on a $24 \times 4$ cylinder for $U = 8$. The pinning field is applied to the edge sites (denoted by the crosses).

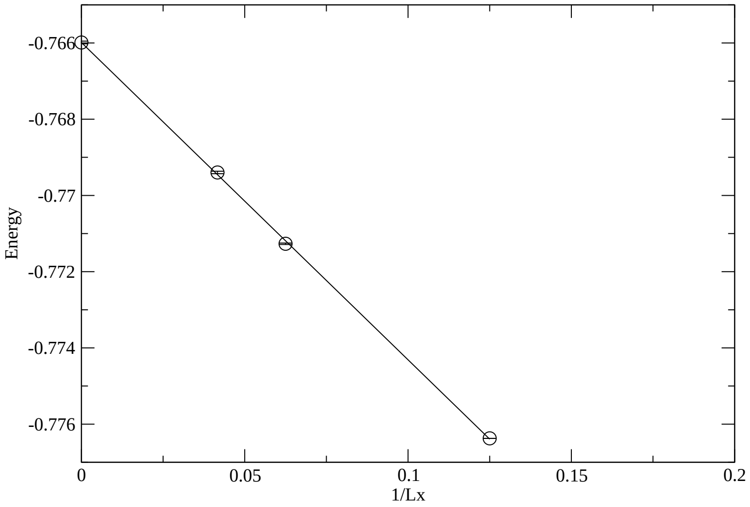


Figure S14: Energy versus $1/L_x$ for width $4$ cylinders.

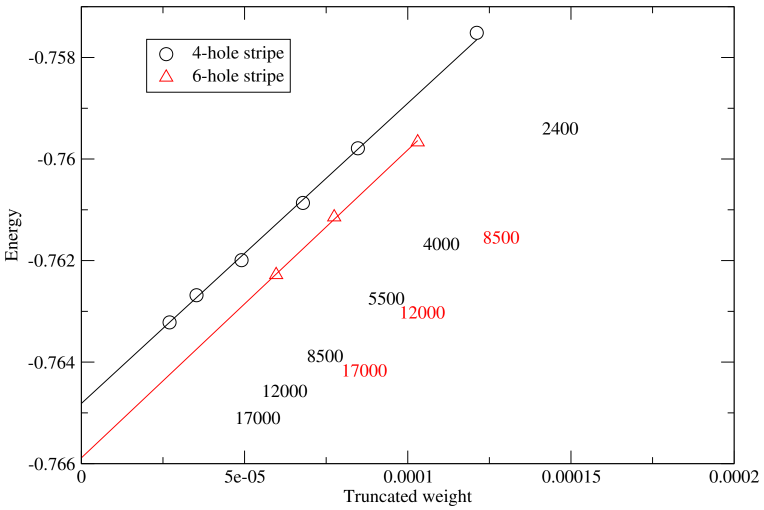


Figure S15: Energy versus truncated weight for wavelength=5 (4-hole stripe) and wavelength=8 (6-hole stripe) states on $32 \times 6$ cylinders with pinning field of strength $|h| = 0.5$ for $U = 8$. The numbers show the bond dimensions of the corresponding points.

lower energy can only be observed when we carefully setup the initial states and extrapolate the energy to zero truncated weight (infinite bond dimension). We show a comparison of energy vs. truncated weight for wavelength $5$ (4-hole stripes) and wavelength $8$ (6-hole stripes) states on $32 \times 6$ cylinders in Fig. S15 as an example.

We show the energies versus $1/L_x$ for the wavelength $5$ and wavelength $8$ states, both with and without pinning fields, in Fig.S16. The spin and hole density expectation values on $32 \times 6$ cylinders are shown in Fig.S17.

### S6.2.4 Width-7 cylinder, horizontal stripe

To access another possible wavelength, we considered width-7 cylinders, on which horizontal stripe states with wavelength 7 can be stabilized (see Fig.S19). We used a product initial state and temporary fields in the first few sweeps, as described in the last section, to stabilize the

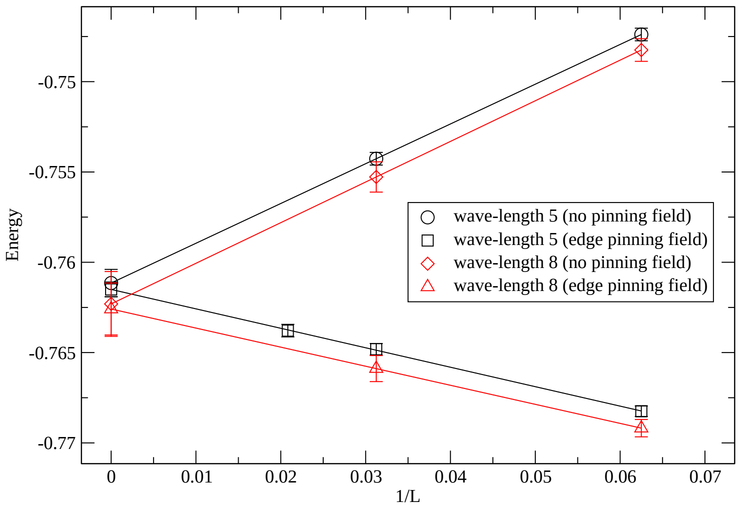


Figure S16: Energy versus $1/L_x$ for the wavelength $5$ and wavelength $8$ states on width-$6$ cylinders for $U = 8$. The wavelength $8$ state has a slightly lower energy.

states. No permanent pinning field was applied. Cylinder sizes of $16 \times 7$, $32 \times 7$, and $48 \times 7$ were considered. The energies for different lengths are shown in Fig.S18. The spin and hole density expectation values are shown in Fig.S19.

#### S6.2.5 Width-6 cylinder, wave length 9

The stripe state with wavelength $9$, where each stripe would contain $8$ holes, is unstable on a width-$6$ cylinder (which means that it will split into $4$-hole stripes with wave length $5$). We therefore provide only a rough estimation of its energy. We forced the holes to be on particular sites by applying strong chemical potentials and magnetic fields throughout the whole system, to form stripes in the first several sweeps up to bond dimension $m = 4000$. We then turned off the field except at the edges, and measured the energy in the following few sweeps where the stripes were not yet completed melted. The finite size energy was estimated by the extrapolation of $m = 7000$ and $m = 9000$ states, with an error bar defined by the difference between the

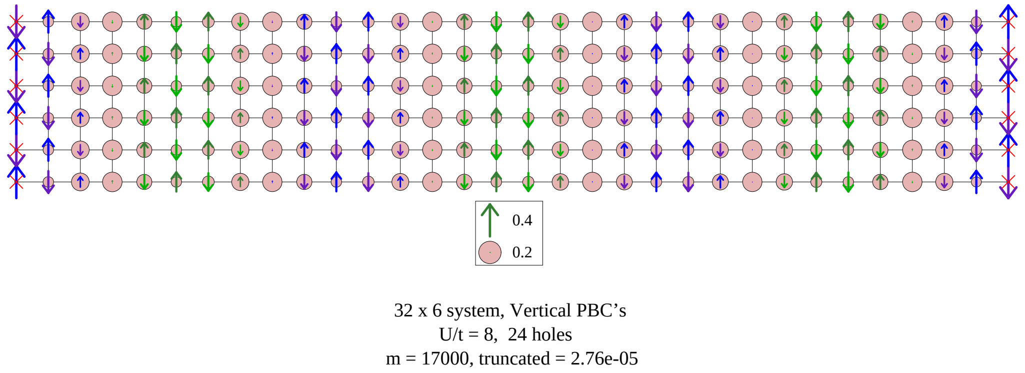


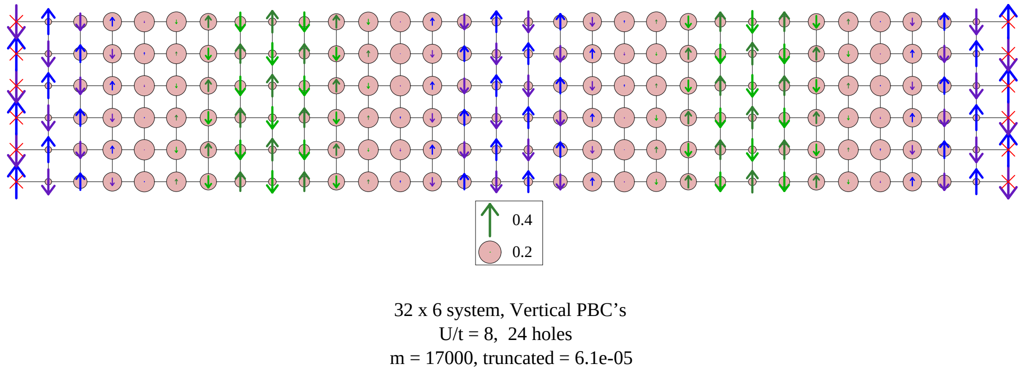


Figure S17: Spin (arrow) and hole density (circle) expectation values of the wavelength $5$ and wavelength $8$ states on $32 \times 4$ cylinders for $U = 8$. The pinning field is applied to the edge sites (denoted by the crosses).

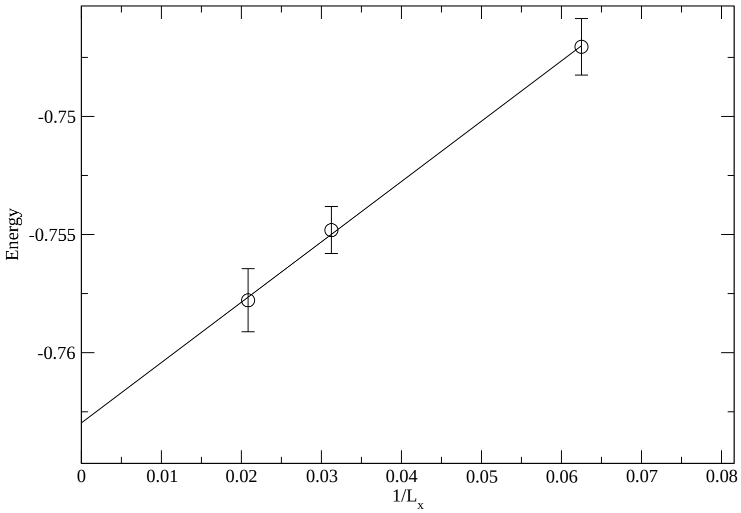


Figure S18: Energy versus $1/L_x$ for horizontal stripe states of wavelength 7 on width-7 cylinders for $U = 8$.

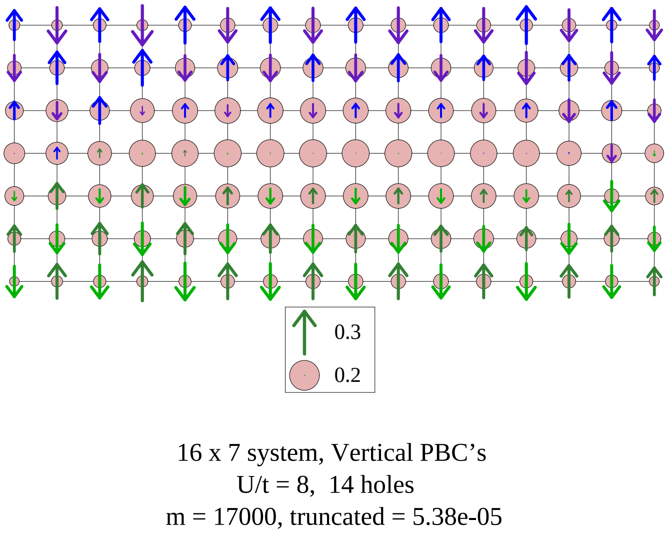


Figure S19: Spin (arrow) and hole density (circle) expectation values for a horizontal stripe state on a $16 \times 7$ cylinder for $U = 8$.

energy of the $m = 9000$ state and the extrapolated energy. The energy of the infinite-length cylinder was estimated from the bulk energy by subtracting the energies of $64 \times 6$ and $32 \times 6$ cylinders. We show the wavelength-9 stripes with $m = 5500$ and $m = 7000$ on a $32 \times 6$ cylinder in Fig.S20.

## S6.3 U=8, Pairing

Since pairing operators break total particle number conservation, we used grand canonical simulations. An additional global chemical potential term $-\mu\hat{N}$ was added to the Hamiltonian, where $\hat{N}$ is the total particle number operator. The chemical potential $\mu$ is tuned such that $\langle\hat{N}\rangle$ is close to $7/8$ of the number of sites (1/8 doping). Defining the singlet pairing operator $\hat{\Delta}^{\dagger}_{ij} \equiv \frac{1}{\sqrt{2}}\left(\hat{c}^{\dagger}_{i\uparrow}\hat{c}^{\dagger}_{j\downarrow} - \hat{c}^{\dagger}_{i\downarrow}\hat{c}^{\dagger}_{j\uparrow}\right)$, and the averaged pairing operator $\hat{D}_{ij} \equiv \frac{1}{2}\left(\hat{\Delta}^{\dagger}_{ij} + \hat{\Delta}_{ij}\right)$, we applied d-wave pairing fields $\mathcal{D}\hat{D}_{ij}$ on the edge bonds, with $\mathcal{D} = 1.0$ for the horizontal bonds and $\mathcal{D} = -1.0$ for the vertical bonds, and measured the pairing order $\Delta_{ij} = \langle\hat{\Delta}_{ij}\rangle$ on each bond for the whole system.

Cylinder sizes of $16 \times 4$ and $32 \times 4$ were considered. For both sizes we used a chemical potential of $\mu = 1.75$, which gave us charge densities of $\sim 0.8751$ for the $16 \times 4$ cylinder and $\sim 0.8756$ for the $32 \times 4$ cylinder, for a bond dimension of $m = 12000$. The truncation error per site was $\sim 6 \times 10^{-6}$ for the $16 \times 4$ cylinder and $\sim 10^{-5}$ for the $32 \times 4$ cylinder. The spin, hole densities, and pairing orders are shown in Fig.S21.

The pairing orders $\Delta_{ij}$ on the bonds where $y = 1$ are shown in Fig.S22 (black circles). The positive parts are for the vertical bonds and the negative parts are for the horizontal bonds, showing the $d$-wave symmetry. For the $16 \times 4$ cylinder, the pairing order strength decays from the edges and has a minimum value $\sim 0.01$ at the center. For the $32 \times 4$ cylinder, the pairing order strength decays from the edges, and then grows to a peak at the center. We also show the extrapolated $\Delta_{ij}$ to zero truncation error in Fig.S22 (red diamond). For the $32 \times 4$ cylinder,

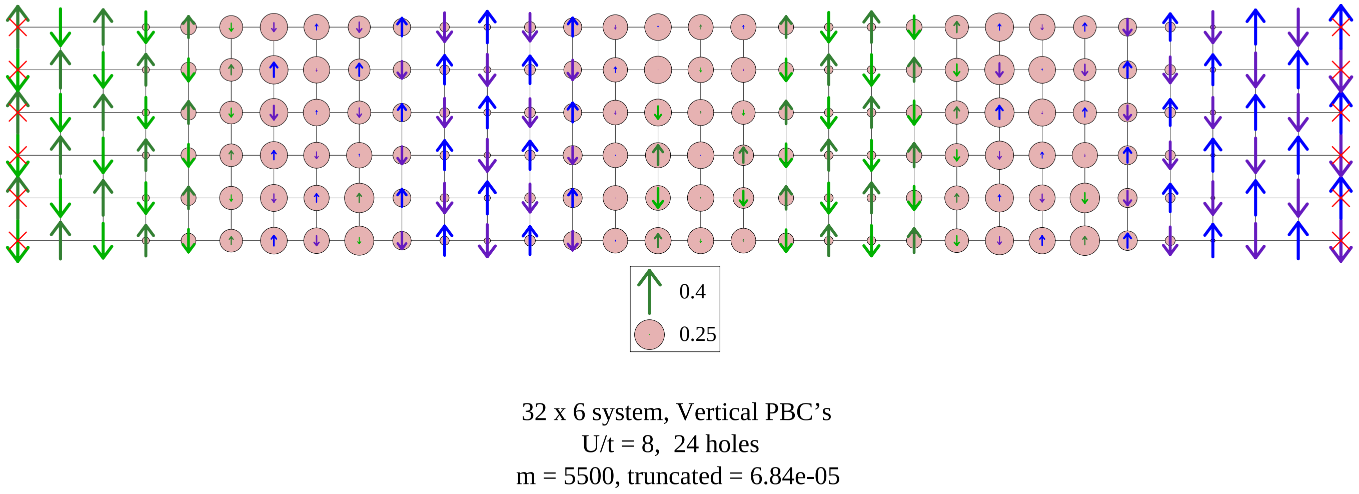


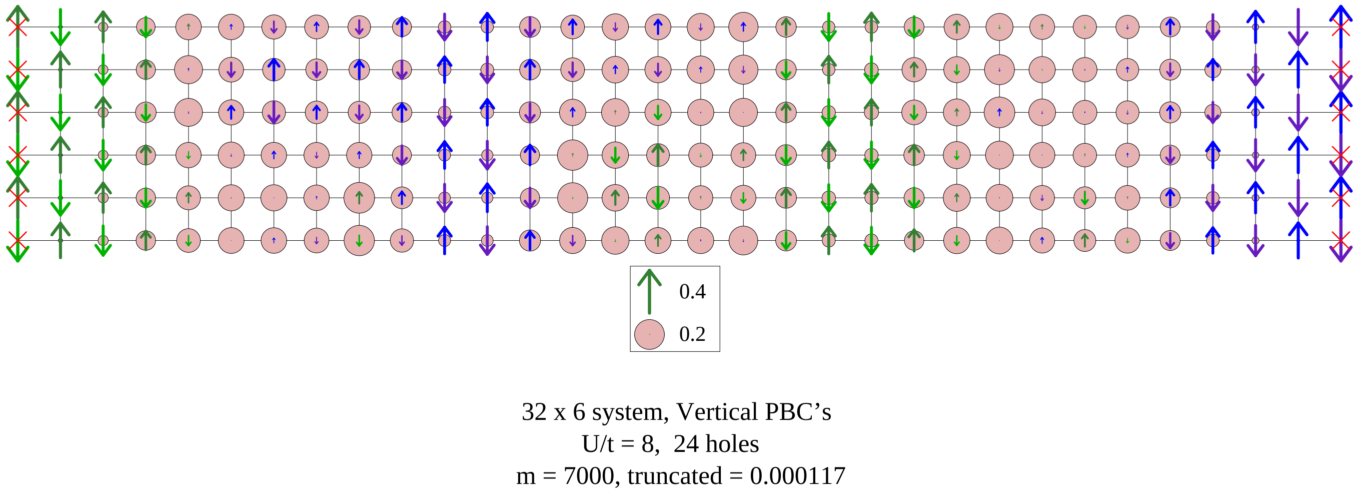


Figure S20: Wave length 9 stripes on a $32 \times 6$ cylinder for $m = 5500$ and $m = 7000$ for $U = 8$.

when the number of states $m$ increases, the pairing strength decreases close to the edges ($x \sim 8$ and 23) and increases in the center, showing the $d$-wave pairing domain. The extrapolations of $\Delta_{ij}$ for the central bonds ($i_x = L_x/2$, $i_y = 1$) are shown in Fig.S23. Again the positive points are for the vertical bonds and the negative points are for the horizontal bonds. We linear extrapolate the last two points, and define the error-bar of extrapolation as $1/4$ of the difference between the last point and the extrapolated value.

To compare the energy with the results from particle number conserved simulations, we computed the bulk energy $E_{\text{bulk}} \equiv [E(N_2) - E(N_2)] / (N_2 - N_1)$ for $N_2 = 32 \times 4$ and $N_1 = 16 \times 4$, where $E(N)$ is the total energy of the system with size $N = L_x L_y$. The bulk energy here is $-0.7639(1)$. This is a little bit higher than the energy $-0.76598(3)$ of the infinite cylinder.

## S6.4 U=12, fixed particle number

Here we show the DMRG results for $U = 12$ and the $1/8$ hole-doped Hubbard model. We consider cylinders with width 4 and 6.

For width 4, we consider the stripes where each stripe contains 2 or 4 holes (stripe fillings $1/2$ and 1), and the mixture of 2-hole and 4-hole stripes. The wavelengths of 2-hole and 4-hole stripes are $\lambda = 4$ and 8 respectively, and the mixed stripes have the wavelengths in between. We thus use the mixture of stripes to estimate the energies of intermediate wavelengths. The mixture of stripes is stabilized by specifying the initial state and by applying pinning fields in the first few sweeps, as before. For the mixture of stripes, we add an extra column to the cylinders to better fit the wavelength, so the doping is not exactly $1/8$ for the finite-length cylinders; however it approaches $1/8$ doping in the extrapolation of the length$\rightarrow \infty$. We found that for width 4 cylinders the mixed stripes with wavelength around $5-6$ have lower energies than the 2-hole and 4-hole stripes, as shown in Fig. S24. The energies of different states are shown in Tab. S9.

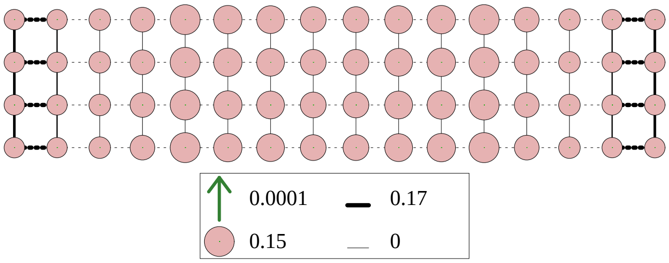


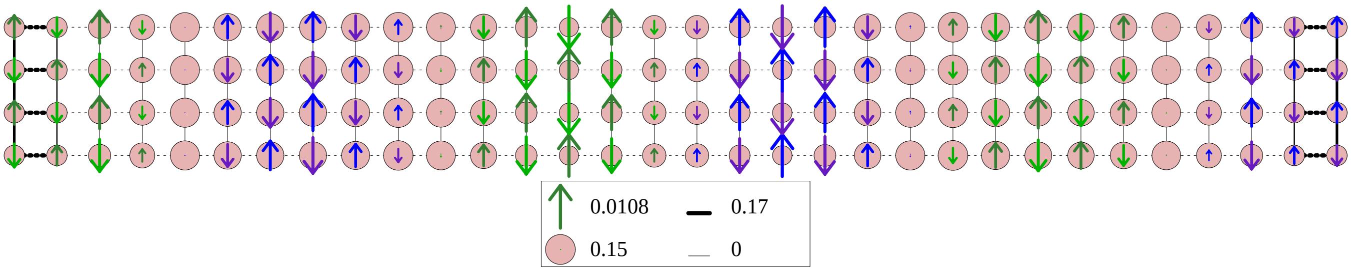


Figure S21: Spin (arrow), hole densities (circles), and pairing order (bonds) in the $16 \times 4$ and $32 \times 4$ cylinders for $U = 8$. The bond widths are proportional to the strengths of the pairing order $\Delta_{ij}$, and the solid lines represent positive signs and dashed lines represent negative signs. The pairing field is applied at the edge bonds, indicated by the thick bonds at the edges.

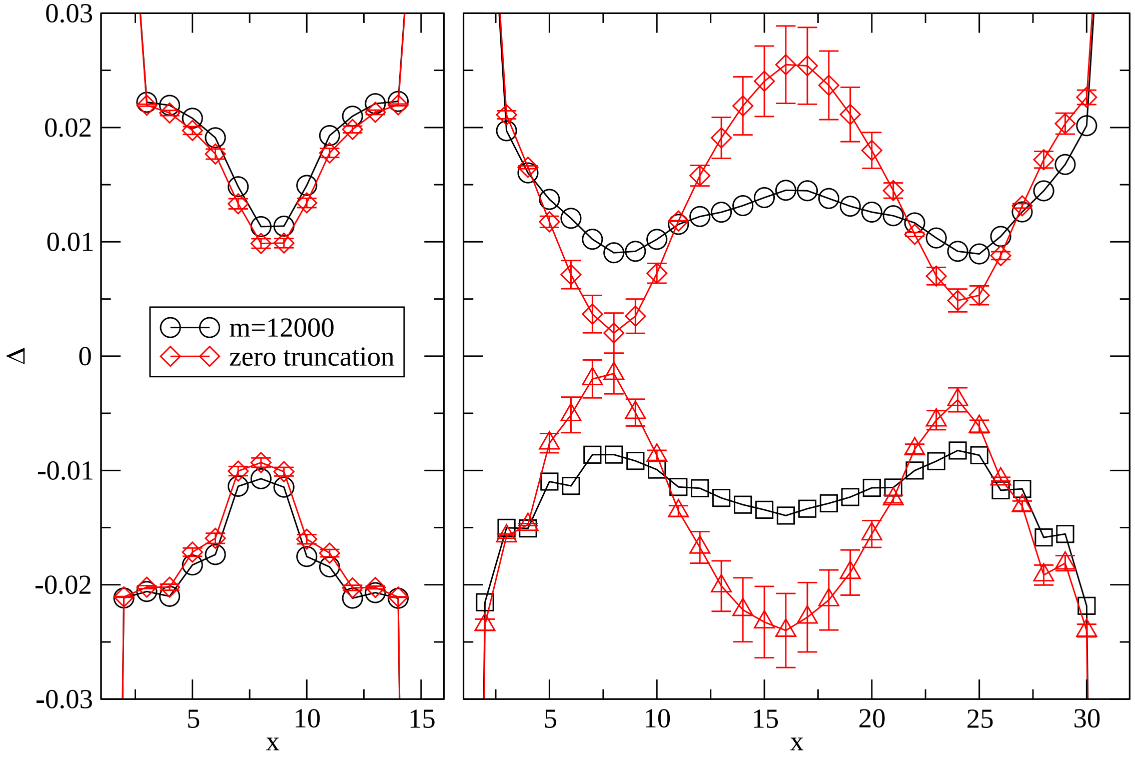


Figure S22: $\Delta_{ij}$ on bonds of $y_i = 1$ for the $16 \times 4$ (left panel) and $32 \times 4$ (right panel) cylinders. The positive parts are for the vertical bonds and the negative parts are for the horizontal bonds, showing the $d$-wave feature. The black circles are measured with bond dimension $m = 12000$, and the red diamonds are extrapolated results to zero truncation error. The error-bars are defined as $1/4$ of the difference between the $m = 12000$ results and the extrapolated results.

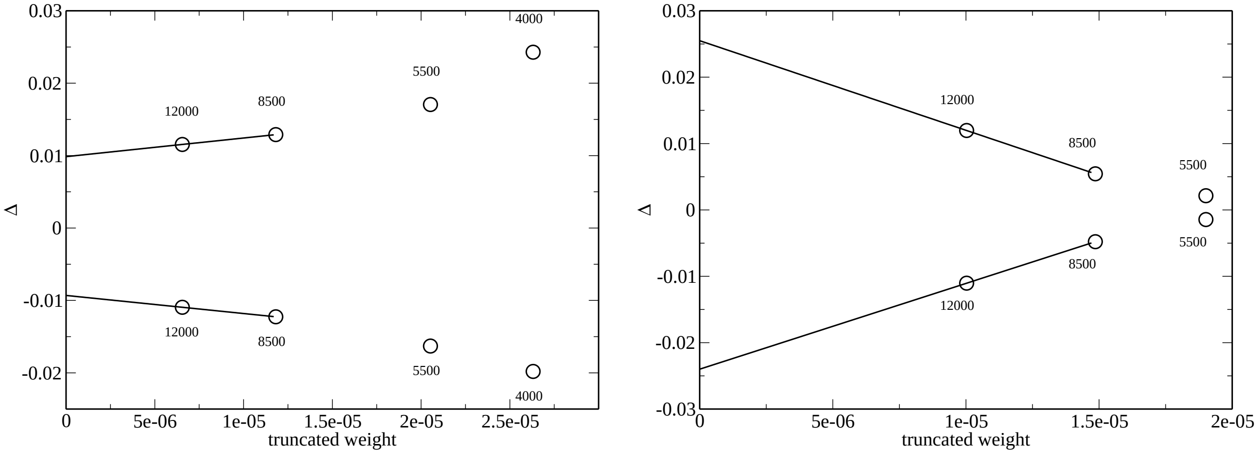


Figure S23: The linear extrapolation of $\Delta_{ij}$ versus truncation errors for the last two sweeps. Left panel: $16 \times 6$ cylinder. Right panel: $32 \times 6$ cylinder. $i_x = L_x/2$ and $i_y = 1$. The positive points are for the vertical bonds ($j_x = i_x, j_y = i_y + 1$) and the negative points are for the horizontal bonds ($j_x = i_x + 1$, $j_y = i_y$). The numbers show the number of states in each sweep.

Similarly, for width $6$, we consider the $4$-hole and $6$-hole stripes (filling $2/3$ and $1$) with wavelengths $\lambda = 5$ and $\lambda = 8$, as well as the mixture of $4$-hole and $6$-hole stripes with wavelengths in between. For width=6 we found that the lowest-energy state is the one with wavelength $8$ (filled stripes), and the wavelength $5$ and mixed stripes have slightly higher energies. The energy extrapolation with $1/L_x$ is shown in Fig S25. The energies of the different stripe states are listed in Tab. S9. We note that the $\lambda = 4$ stripe from the mixing of $2$-hole and $4$-hole stripes is not stable in the DMRG simulations, so the energy is only a rough estimate.

We note that, as mentioned in S6.2.3 for the $U = 8$ case, we compare the energies after the extrapolation to zero truncated weight (infinite bond dimension). In Fig. S26 we show the energy versus truncated weight comparison of the wavelength $5$ ($4$-hole stripe) and wavelength $8$ ($6$-hole stripe) states on $32 \times 6$ cylinders. Note that with fixed bond dimension the wavelength $5$ state has lower energy. Only after extrapolation, can it be seen that the wavelength $8$ state actually has a lower energy.

We show the spin and hole expectation values of the mixture of $2$-hole and $4$-hole stripes on

| width 4 | |
|---|---|
| 2h,$\lambda = 4$ | $-0.641379 \pm 5.2e-05$ |
| 4h,$\lambda = 8$ | $-0.641677 \pm 0.00023$ |
| 2+4,$\lambda \sim 6$ | $-0.642853 \pm 0.00021$ |
| 2+2+4+4,$\lambda \sim 6$ | $-0.642707 \pm 0.00022$ |
| 2+4+4+2,$\lambda \sim 6$ | $-0.642507 \pm 0.00018$ |
| 2+2+4+2+2,$\lambda \sim 4.8$ | $-0.642692 \pm 0.00019$ |

| width 6 | |
|---|---|
| 4h,$\lambda = 5$ | $-0.64148 \pm 0.00059$ |
| 6h,$\lambda = 8$ | $-0.6438 \pm 0.0019$ |
| 4+4+6+4,$\lambda \sim 6$ | $-0.6418$±$0.0013$ |
| 4+6+4+6+4,$\lambda \sim 6.5$ | $-0.6420 \pm 0.0016$ |
| 2+4,$\lambda \sim 4$ | $-0.6383 \pm 0.0026$ |

Table S9: Energies of stripe states with different wavelengths for $U = 12$ on infinite-length cylinders.

a $17 \times 4$ cylinder in Fig. S27 as an example of the mixed stripes.

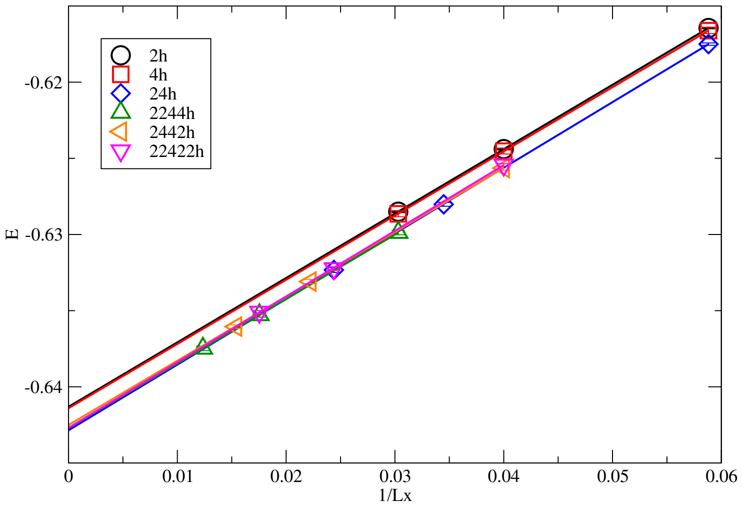


Figure S24: Energy extrapolations vs. $1/L_x$ for the extra-column width-4 cylinders for the 2-hole, 4-hole, and the mixing stripes for $U = 12$. The mixing stripes have lower energies.

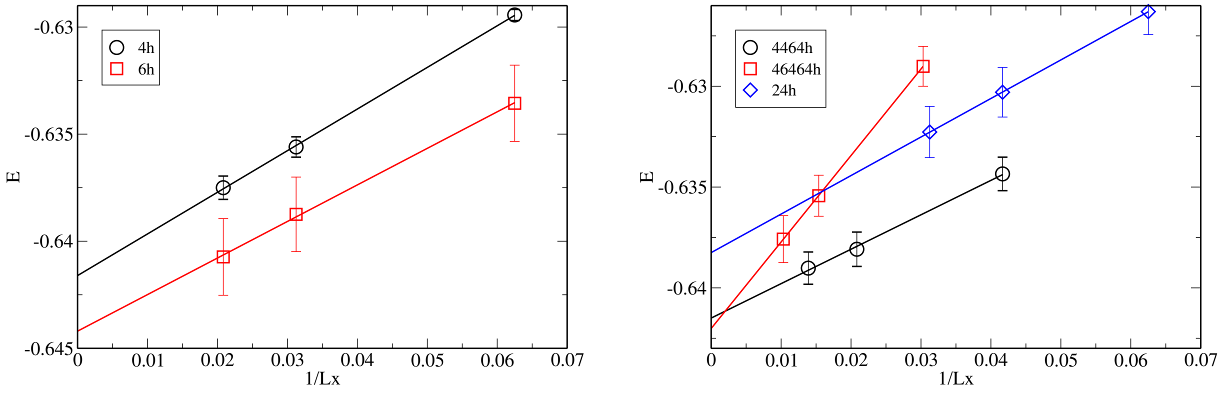


Figure S25: Energy extrapolations vs. $1/L_x$ for the 4-hole, 6-hole (left panel), and the mixing stripes (right panel) for width-6 cylinders for $U = 12$.

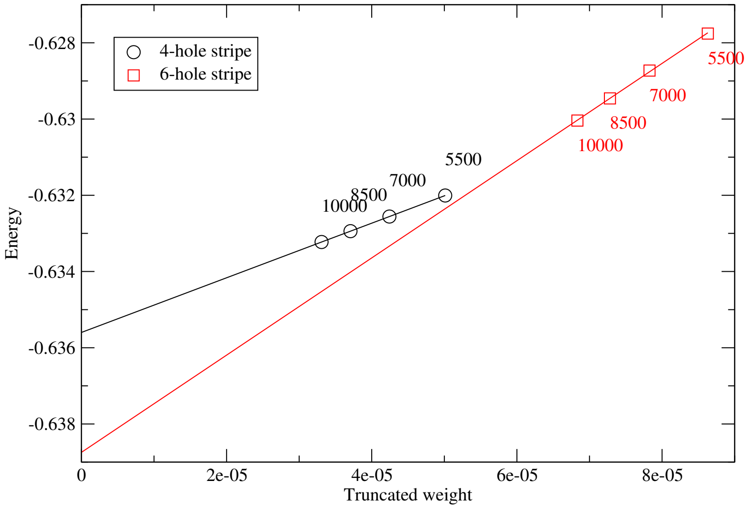


Figure S26: Energy versus truncated weight for wavelength=5 (4-hole stripe) and wavelength=8 (6-hole stripe) states on $32 \times 6$ cylinders for $U = 12$. The numbers show the bond dimensions of the corresponding points.

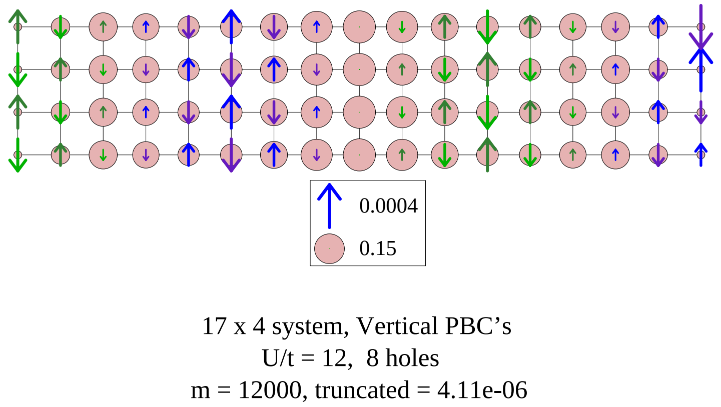


Figure S27: Spin (arrow) and hole densities (circles) of mixture of 2-hole and 4-hole stripes on a $17 \times 4$ cylinder for $U = 12$. There are two of 2-hole stripes on the two sides and a 4-hole stripe in the center.

# S7 Hybrid-basis DMRG

## S7.1 Details of the hybrid-basis DMRG calculations

We use a cylinder geometry with cylinder length $L_x$, width $L_y$, with open boundary conditions in the longitudinal (long) axis, and periodic boundary conditions (PBC) or anti-periodic boundary conditions (APBC) in the transverse direction.

We used the density matrix renormalization group (DMRG) algorithm in a mixed–real-momentum-space (hybrid) representation (*34*). The hybrid-space DMRG algorithm uses a real-space representation in the longitudinal cylinder direction and a momentum-space representation in the transverse direction. The additional transverse-momentum quantum number grants us a speedup over real-space DMRG that grows with the width of the cylinder. For width-6 Hubbard cylinders, the hybrid-space algorithm is approximately 20 times faster than its real-space counterpart.

In order to obtain the ground-state energy for fixed $L_y$, we performed consecutive extrapolations first in the DMRG truncation error $\Delta\xi$ (Fig. S28) and then in the inverse cylinder length $1/L_x$ (Fig. S29). The ground-state energies at $U/t = 8.0$ for all available combinations of $L_y$, $L_x$, boundary conditions, and different stripe patterns (i.e., wavelengths), are given in Table S10.

For width $4$, we found stable ground states with $4$ holes per stripe for PBC and APBC. For width-$6$ cylinders with PBC, we found two stable states with $4$ and $6$ holes per stripe, with the $6$-hole stripe pattern being energetically favorable for all cylinder lengths. Thus, for width-4 and width-6 cylinders, we found charge-density stripes with a wavelength of 8 sites for the ground state. For width $6$ with APBC, we were not able to effectively stabilize the stripe patterns. For width $8$, we did not achieve sufficient convergence in the energy, despite using up to $35\,000$ states.

In order to directly target and stabilize different stripe configurations on width-6 cylinders

with PBC, we used a sine-shaped pinning field coupled to the local charge density $n_{x\,y\,\sigma}$,

$$P = \sum_{x\,y\,\sigma} A\,\cos(k_x\,x\,+\,\phi_0)\,n_{x\,y\,\sigma}\,, \tag{S2}$$

with suitable amplitude $A$, wave vector $k_x$, and phase $\phi_0$. The contribution to the ground-state energy, $\langle\Psi_0|P|\Psi_0\rangle$, is subtracted after the DMRG calculation. We found a field amplitude of $A = 0.01$ to be sufficient to stabilize the different stripe patterns and to improve the convergence of the DMRG algorithm.

The stripe patterns in the charge density distribution,

$$\overline{n}_{\text{tot.}}(x) = \sum_{k_y\,\sigma}\langle\Psi|n_{x\,k_y\,\sigma}|\Psi\rangle\,, \tag{S3}$$

can be measured directly and are shown in Figure S30. Depending on the wavelength of the charge density stripes, we also found corresponding peaks in the charge structure factor

$$S_C(\mathbf{q}) = \frac{1}{N}\sum_{\mathbf{r}\,\mathbf{r}'} e^{\mathrm{i}\,\mathbf{q}(\mathbf{r}-\mathbf{r}')}\,\langle n_{\mathbf{r}}\,n_{\mathbf{r}'}\rangle\,, \tag{S4}$$

with $n_{\mathbf{r}} = n_{\mathbf{r}\uparrow} + n_{\mathbf{r}\downarrow}$, shown in Fig. S31 for 32×4 and 32×6 cylinders; wavelength $8$ ($5.\overline{3}$) stripes result in peaks at momenta $k_x = \pm 4/16\,\pi$ ($k_x = \pm 6/16\,\pi$). Figure S32 shows the corresponding spin-structure factor

$$S_S(\mathbf{q}) = \frac{1}{N}\sum_{\mathbf{r}\,\mathbf{r}'} e^{\mathrm{i}\,\mathbf{q}(\mathbf{r}-\mathbf{r}')}\,\langle m_{\mathbf{r}}\,m_{\mathbf{r}'}\rangle\,, \tag{S5}$$

with $m_{\mathbf{r}} = n_{\mathbf{r}\uparrow} - n_{\mathbf{r}\downarrow}$, which shows peaks at $k_x = (1 \pm 2/16)\pi$ $[k_x = (1 \pm 3/16)\pi]$. These peaks correspond to the antiferromagnetic order with a modulation / phase-shift of wavelength $16$ ($10.\overline{6}$). Due to the momentum-space representation in the transverse direction, we could not measure the stripes in the staggered-spin density distribution directly (applying a corresponding field would break the translational invariance).

Finally, we have also measured the decay of the equal-time pair-field correlations

$$D_{\mathrm{y,y}}(\mathbf{r},\mathbf{r}') = \langle\Delta^\dagger_{\mathrm{y}}(\mathbf{r})\,\Delta_{\mathrm{y}}(\mathbf{r}')\rangle\,, \tag{S6}$$

with pair-field creation operator $\Delta_{\mathrm{y}}^{\dagger}(x,y) = \frac{1}{\sqrt{2}}\,(c^{\dagger}_{x\,y+1\uparrow}\,c^{\dagger}_{x\,y\downarrow} - c^{\dagger}_{x\,y+1\downarrow}\,c^{\dagger}_{x\,y\uparrow})$, as a function of the longitudinal distance for width-$4$ cylinders (Fig. S33). For small distances $l_x$, the correlations decay roughly as $l_x^{-2}$, before crossing over to an exponential decay for larger $l_x$. The different regimes can be highlighted by choosing a log-log or linear-log scale (Fig. S33 and S34).

Compared to chains or 2-leg ladders the number of states seems insufficient to exactly represent the long-range pair-field correlations for larger correlation lengths. For width $6$, the situation becomes even worse, and the exponential decay is dominant at all length scales.

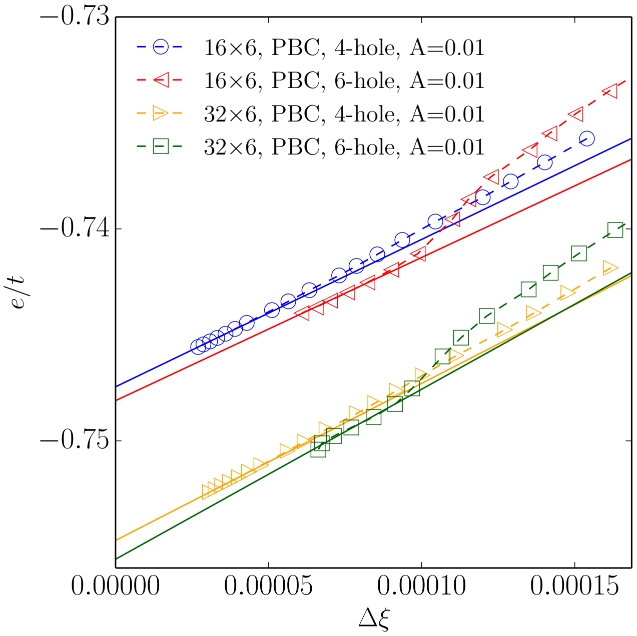


Figure S28: (Color online) Truncation-error extrapolation of the ground-state energy for $16\times6$ and $32\times6$ cylinders at $U/t = 8.0$ with periodic boundary conditions in transverse direction for 4-hole and 6-hole stripe patterns.

| dimensions $L_x \times L_y$ | boundary conditions | longitudinal wavelength | holes per stripe | pinning field amplitude | $m_{\max}$ | $e/t$ |
|---|---|---|---|---|---|---|
| $16\times4$ | PBC | $8.0$ | $4$ | $0$ | $30000$ | $-0.75114(2)$ |
| $16\times4$ | APBC | $8.0$ | $4$ | $0$ | $30000$ | $-0.74712(2)$ |
| $32\times4$ | PBC | $8.0$ | $4$ | $0$ | $30000$ | $-0.75841(2)$ |
| $32\times4$ | APBC | $8.0$ | $4$ | $0$ | $30000$ | $-0.75382(3)$ |
| $48\times4$ | PBC | $8.0$ | $4$ | $0$ | $27500$ | $-0.76079(2)$ |
| $48\times4$ | APBC | $8.0$ | $4$ | $0$ | $30000$ | $-0.75604(4)$ |
| $64\times4$ | PBC | $8.0$ | $4$ | $0$ | $25000$ | $-0.7621(5)$ |
| $64\times4$ | APBC | $8.0$ | $4$ | $0$ | $27500$ | $-0.75725(6)$ |
| $\infty\times4$ | PBC | $8.0$ | $4$ | $0$ | - | $-0.7657(3)$ |
| $\infty\times4$ | APBC | $8.0$ | $4$ | $0$ | - | $-0.76057(7)$ |
| $16\times6$ | PBC | $8.0$ | $6$ | $0.01$ | $35000$ | $-0.7481(2)$ |
| $16\times6$ | PBC | $5.\overline{3}$ | $4$ | $0.01$ | $35000$ | $-0.74745(2)$ |
| $32\times6$ | PBC | $8.0$ | $6$ | $0.01$ | $35000$ | $-0.7556(7)$ |
| $32\times6$ | PBC | $5.\overline{3}$ | $4$ | $0.01$ | $35000$ | $-0.754702(3)$ |
| $48\times6$ | PBC | $8.0$ | $6$ | $0.01$ | $35000$ | $-0.7577(3)$ |
| $48\times6$ | PBC | $5.\overline{3}$ | $4$ | $0.01$ | $27500$ | $-0.75727(1)$ |
| $64\times6$ | PBC | $8.0$ | $6$ | $0.01$ | $35000$ | $-0.7591(2)$ |
| $64\times6$ | PBC | $5.\overline{3}$ | $4$ | $0.01$ | $25000$ | $-0.75842(4)$ |
| $\infty\times6$ | PBC | $8.0$ | $6$ | $0.01$ | - | $-0.7627(5)$ |
| $\infty\times6$ | PBC | $5.\overline{3}$ | $4$ | $0.01$ | - | $-0.76210(5)$ |

Table S10: Zero-truncation-error extrapolated ground-state energies of Hubbard cylinders at $U/t = 8.0$ and $n = 0.875$ filling for different stripe patterns, system sizes, and transverse boundary conditions. The given wavelength describes the charge-density waves. For width 6, a pinning field was used to stabilize the different stripe configuration; the energy contribution of the pinning-field was subtracted afterwards.

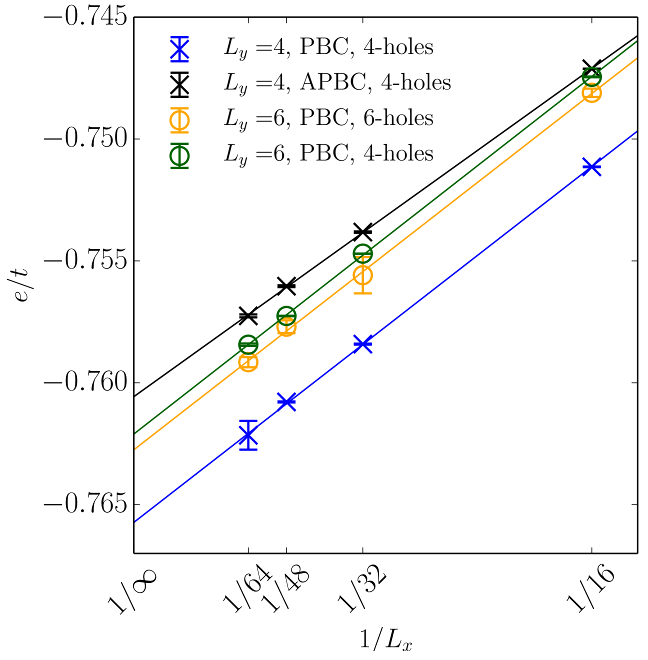


Figure S29: (Color online) Cylinder-length extrapolation of the ground-state energy per cite for cylinders with width $4$ and $6$ at $U/t = 8.0$.

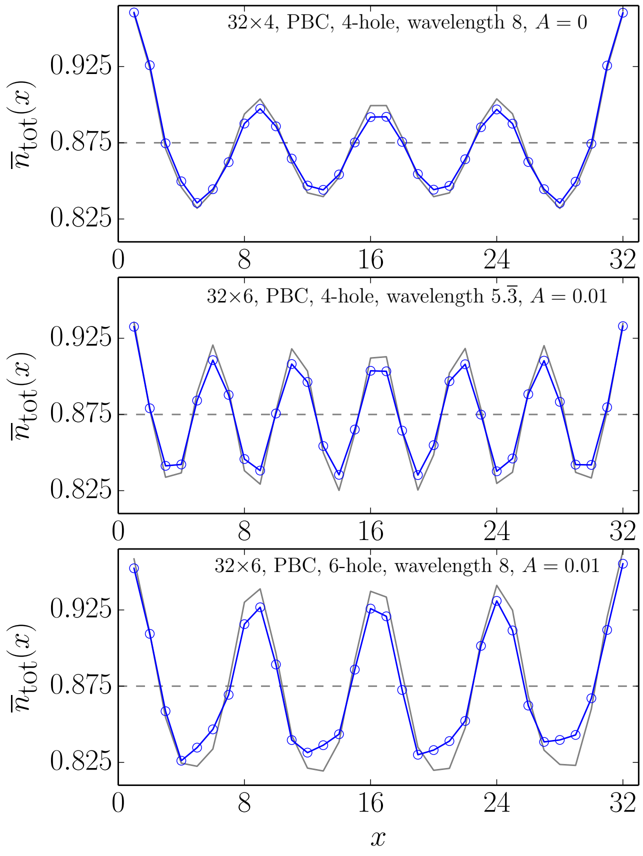


Figure S30: (Color online) Charge density distribution for the $32{\times}4$ and $32{\times}6$ Hubbard model at $U/t = 8.0$ and $n = 0.875$ filling. The density calculated during the last DMRG sweep is plotted in gray, and the zero truncation error extrapolation is plotted in blue. For width $6$ a pinning field with amplitude $0.01$ was used to stabilize the stripes.

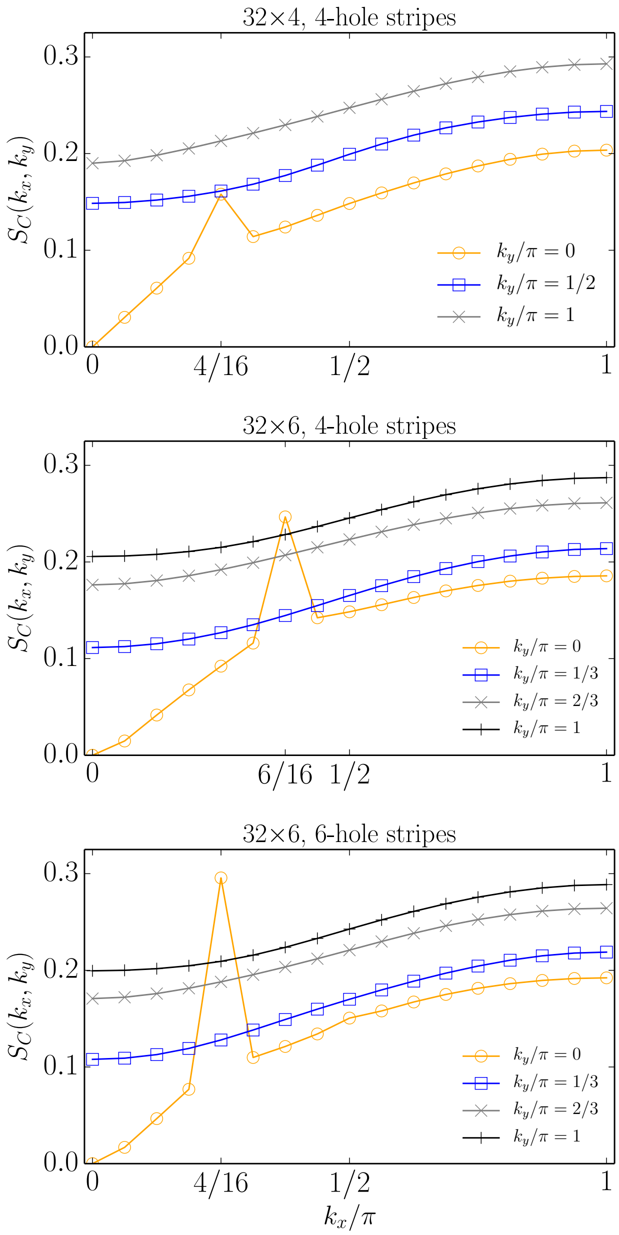


Figure S31: (Color online) Charge structure factor $S_C(\mathbf{k})$ for width-4 cylinders with 4-hole stripes (top), width-6 cylinders with 4-hole stripes (middle), and width-6 cylinder with 6-hole stripes (bottom) at $U/t = 8.0$. The length of the cylinders in all cases is 32. We show only momenta points $0 \leq k_{x/y} \leq \pi$.

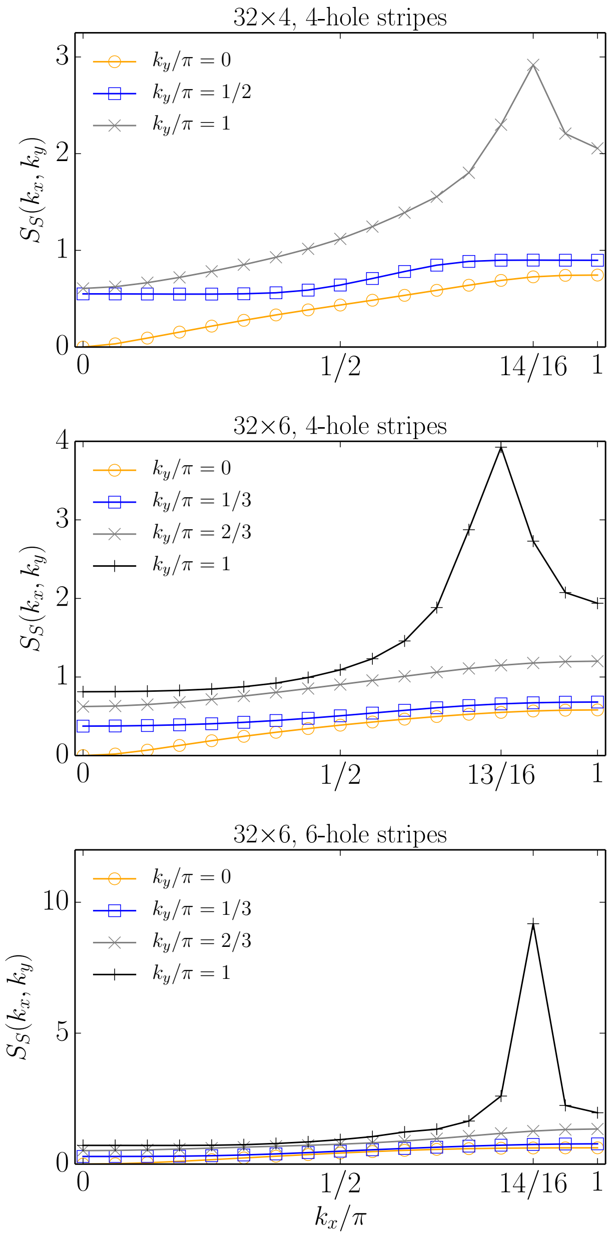


Figure S32: (Color online) Spin structure factor $S_S(\mathbf{k})$ for width-4 cylinders with 4-hole stripes (top), width-6 cylinders with 4-hole stripes (middle), and width-6 cylinder with 6-hole stripes (bottom) at $U/t = 8.0$. The length of the cylinders in all cases is 32. We show only momenta points $0 \leq k_{x/y} \leq \pi$.

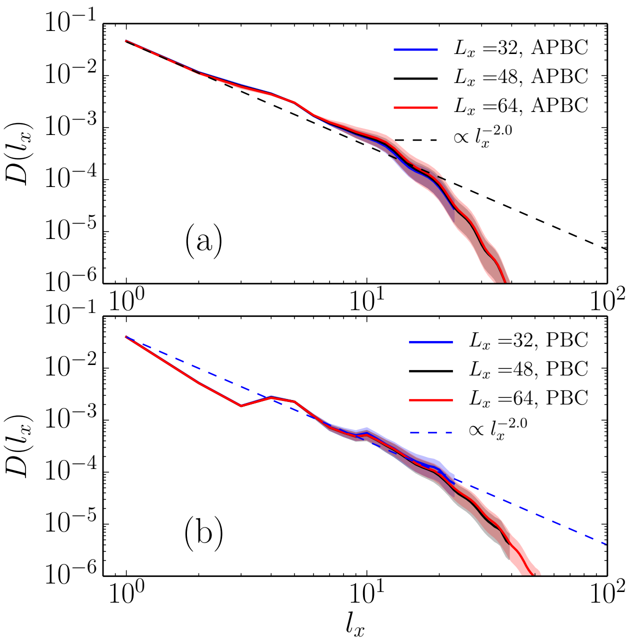


Figure S33: (Color online) Equal time pair-field correlations in longitudinal direction for width-4 cylinders at $U/t = 8.0$ with cylinder length 32, 48, and 64, 4-hole (wavelength-8) stripes, and anti-periodic (top) and periodic (bottom) boundary conditions.

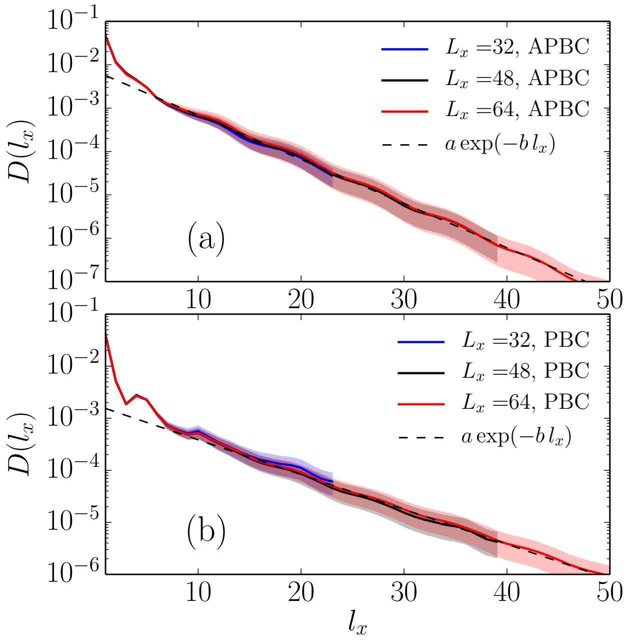


Figure S34: (Color online) Equal time pair-field correlations as in Fig. S33, but on a linear $x$-axis.

# S8 iPEPS

## S8.1 Details of the iPEPS calculations

An infinite projected entangled-pair state (iPEPS) (*37, 39, 54*) (also called a tensor product state (*38, 55*)) is an efficient variational tensor network ansatz for two-dimensional states in the thermodynamic limit which obeys an area law of the entanglement entropy (*56*). The ansatz consists of a supercell of tensors which is periodically repeated on a lattice, with one tensor per lattice site. Each tensor has a physical index which carries the local Hilbert space of a lattice site and four auxiliary indices which connect to the nearest-neighboring tensors on a square lattice. Each auxiliary index has a certain dimension $D$, called the bond dimension, with which the accuracy of the ansatz (the number of variational parameters) can be controlled in a systematic way. An iPEPS with $D = 1$ corresponds to a product state, and by increasing $D$ entanglement can be systematically added. In the present work we used bond dimensions up to $D = 16$ corresponding to highly-entangled states.

For translationally invariant states a supercell with only a single tensor can be used. If the translational symmetry is spontaneously broken a supercell compatible with the symmetry breaking pattern is needed. For example, a Néel ordered state requires a supercell with two different tensors $A$ and $B$ (one for each sublattice), or a stripe state with period 5 requires a $5 \times 2$ (or $2 \times 5$) supercell with 10 independent tensors. A diagonal stripe state with period $\frac{L}{\sqrt{2}}$ can be obtained in a $L \times L$ rectangular supercell, or more efficiently by using a $L \times 1$ supercell with $L$ different tensors and translation vectors $v_1 = (L, 0)$, $v_2 = (1, 1)$. By running simulations with different supercell sizes we can obtain different competing low-energy states. In order to determine which of these competing low-energy states corresponds to the true ground state a systematic analysis of the energy as a function of $D$ is required. Here we used the extrapolation technique from Ref. (*57*) in which the energy is plotted as a function of the so-called truncation

error $w$ in the simulation, and then the extrapolation to the $w \to 0$ limit is taken to determine the energy of each of the competing states. While in 2D it is theoretically unknown how the energy depends on $w$, several benchmarks (*57*) have empirically shown that an accurate estimate can be used using a polynomial fit.

In this work the optimization of the tensors has been done using an imaginary time evolution based on the so-called full update (*58*) (or fast-full update (*59*)), which is more accurate than the simple update approach (*60*). Observables are evaluated by contracting the two-dimensional tensor network in a controlled, approximate way, using a variant (*18, 61*) of the corner-transfer matrix (CTM) method (*62, 63*). The accuracy of the contraction is controlled by the "boundary" dimension $\chi$, which we choose large enough such that the resulting error is small (compared to the effect of the finite $D$). To increase the efficiency we make use of Abelian symmetries (*64, 65*). Fermionic statistics are taken into account following the formalism explained in Refs (*58, 66*).

## S8.2 iPEPS results

We have focussed on studying the competition of the states shown in Fig. S35, including uniform, vertical width-5 (W5), width-7 (W7), width-8 stripes (W8), and a diagonal stripe state. We find all stripes to be site-centered, not bond-centered. The W5 and W7 stripes exhibit coexisting superconducting order together with CDW and SDW order. The W8 stripe and the diagonal stripe have a period-8 in the CDW order and period-16 in the SDW order. Both states exhibit a filling of exactly one hole per unit length at which superconductivity is vanishing. The typical magnitudes of the local magnetic moments and hole densities of the stripes are given by the black and red numbers in Fig. S35, respectively.

In Fig. S36 we present the results for the energy of these competing states, plotted as a function of the inverse bond dimension and the truncation error $w$ (*57*). In order to estimate

the energy of each state in the exact limit we extrapolated the data as a function of $w$ using a third order polynomial. This yields the following estimates for the energies per site, sorted in descending order: $E_s^{uniform} = -0.7555$, $E_s^{diagonal} = -0.7577$, $E_s^{W7} = -0.7620$, $E_s^{W5} = -0.7637$, and $E_s^{W8} = -0.7663$. By averaging over several fits using different ranges of data points we obtain: $E_s^{uniform} = -0.7560 \pm 0.0025$, $E_s^{diagonal} = -0.7581 \pm 0.0014$, $E_s^{W7} = -0.7629 \pm 0.0026$, $E_s^{W5} = -0.7632 \pm 0.0018$, and $E_s^{W8} = -0.7673 \pm 0.0020$.

In summary, we find that the width-8 stripe is energetically favored for $U/t = 8$ and doping $\delta = 1/8$.

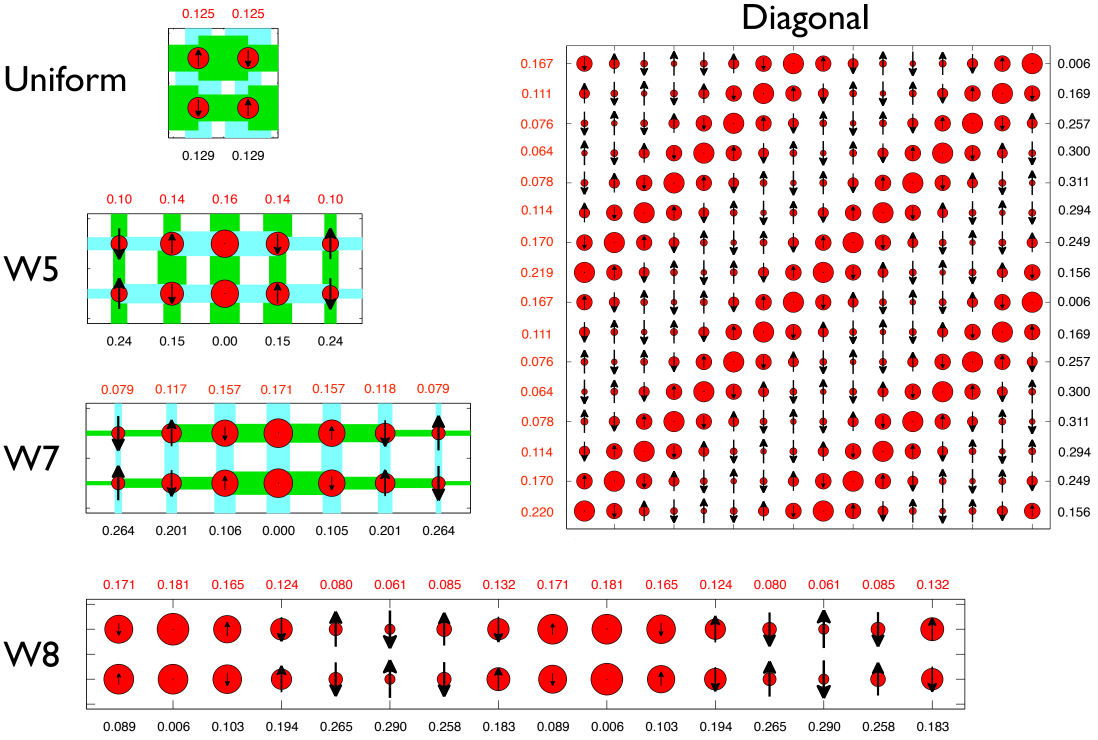


Figure S35: Several competing stripe states obtained with iPEPS for $U/t = 8$, $n = 1/8$. The diameter of the red dots (length of the arrows) is proportional to the local hole density (local magnetic moment). The red numbers indicate the hole density, the black numbers the local magnetic moment, averaged over the sites in a column (on a diagonal in case of the diagonal stripe). The width of a bond between two sites scales with the nearest-neighbor singlet pairing amplitude on the corresponding bond with different sign in horizontal and vertical direction illustrated by the two different colors. The width-5 (W5) and width-7 stripes (W7) have coexisting CDW, SDW, and superconducting order. The width-8 stripe has a period-8 in the CDW order and period-16 in the SDW order, and vanishing superconductivity. The diagonal stripe state also has vanishing superconducting order. The pictures have been obtained with bond dimension $D = 16$, except for the diagonal stripe state ($D = 11$).

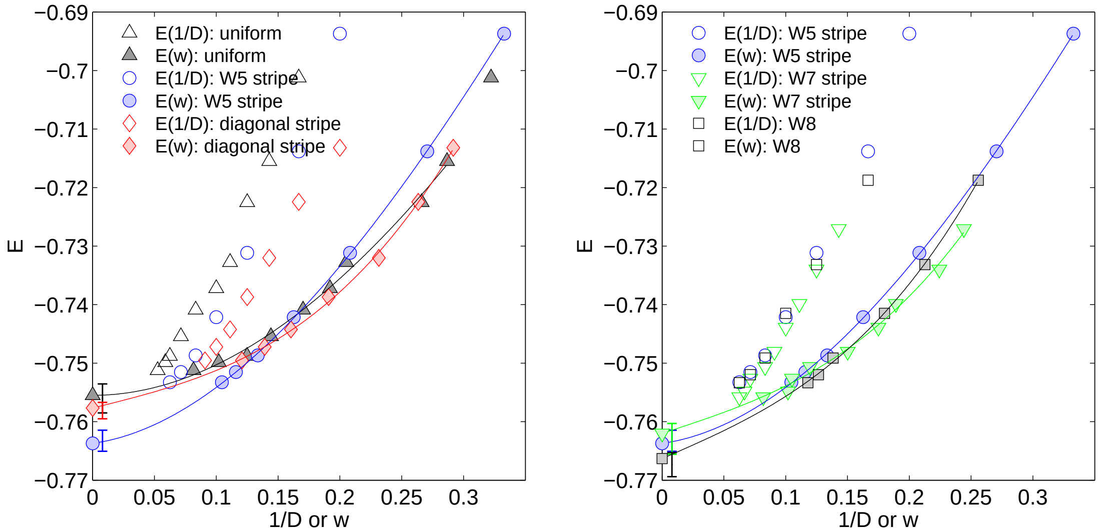


Figure S36: iPEPS results of the energies of the competing states shown in Fig. S35. The data is plotted as a function of $1/D$ (open symbols) and as a function of the truncation error (filled symbols). The W5-stripe is shown in both panels as a reference. The W8 stripe exhibits the lowest extrapolated energy.

# S9 DMET

## S9.1 Details of the DMET calculations

Density matrix embedding theory (DMET) is a wavefunction-based cluster embedding technique that aims to reproduce the boundary entanglement of an impurity cluster using a set of bath sites. Given an impurity cluster of $N_c$ sites, DMET maps a large $L \times L$ lattice to an impurity model through the Schmidt decomposition of an auxiliary lattice wavefunction. The auxiliary lattice wavefunction is usually taken to be of fermionic Gaussian form, i.e. a Slater determinant or BCS state, the ground-state of a quadratic lattice Hamiltonian. The impurity model is then solved with exact or quasi-exact methods such as Lanczos or DMRG to yield an impurity wavefunction. The one-body density matrix of the impurity model and the lattice wavefunction are matched to improve a quadratic correlation potential that is added to the lattice Hamiltonian, which results in a new lattice wavefunction. This process of correlation potential fitting is done self-consistently to optimize the lattice wavefunction and the description of the boundary entanglement. At self-consistency, expectation values both in the cluster and outside can be evaluated using the impurity wavefunction (*19, 36*).

In this work, we use $L = 160$ as the linear dimension of the auxiliary lattice, so finite size errors in the auxiliary lattice wavefunction are negligible. We allow the correlation potential, and thus the impurity and auxiliary wavefunctions, to break spin and particle number symmetry. The calculations are similar to those in Ref. (*19*), but a larger number of impurity cluster sizes, shapes and boundary conditions were explored. Various shapes of impurity clusters are used to accommodate uniform $d$-wave order, vertical and diagonal stripes. The shapes of the clusters are summarized in Fig. S37. We do not attempt to do extrapolation of cluster size in this work as in Refs. (*19, 67*) but compare the energies of different clusters directly. This is making an implicit assumption that the TDL is close to the finite cluster energy, and this lack of TDL extrapolation

is the main systematic error. In our experience, however, it is reasonable to directly compare energies of clusters of the same orientation and family (e.g. $L \times 2$), which is confirmed in this work by comparison with the other techniques.

$\lambda \times 2$ cells [Fig. S37(a)] are used to study vertical stripes with odd wavelengths. As the AF order has a $\pi$-phase shift at the domain wall, the AF order is commensurate with the cell size. For even-wavelength stripes, the setup is similar, however, to support a single domain wall, it is necessary for the spin wavelength to be twice that of the charge wavelength. To allow this, rather than using a large cluster of size $2\lambda \times 2$, we modify the way the correlation potential is added to the lattice wavefunction, i.e. by swapping the spin channels between neighbouring cells in the longitudinal direction [Fig. S37(c)], so translation by a unit cell gives a time reversal, $n_{i\uparrow} \to n_{i\downarrow}$. Specifically, the local correlation potential in this case is written as

$$u = \sum_{C_1} \sum_{i,j \in C_1} (\sum_{\sigma} u_{ij\sigma} a^{\dagger}_{i\sigma} a_{j\sigma} + \Delta_{ij} a^{\dagger}_{i\uparrow} a^{\dagger}_{j\downarrow} + c.c.) + \sum_{C_2} \sum_{i,j \in C_2} (\sum_{\sigma} u_{ij\bar{\sigma}} a^{\dagger}_{i\sigma} a_{j\sigma} + \Delta'_{ij} a^{\dagger}_{i\uparrow} a^{\dagger}_{j\downarrow} + c.c.) \tag{S7}$$

where $C_1$ and $C_2$ label even and odd cells along the longitudinal $x$ direction. Both $\Delta' = \pm\Delta$ possibilities are tested in our calculations, because we cannot determine the phase factor associated with the transformation

$$a_{i\uparrow} \to a_{i+R,\downarrow}, a_{i\downarrow} \to \pm a_{i+R,\uparrow}.$$

where the $R$ denotes translation by a unit cell. As shown in the results, neither parameterization results in finite pairing order in the ground-state of even wavelength stripes.

We also use the tilted clusters in Fig. S37(b) to accommodate diagonal stripes. As the finite-size effects are different in regular and tilted clusters, we use both $2 \times 2$ and $2\sqrt{2} \times \sqrt{2}$ clusters to obtain the uniform $d$-wave state, to estimate the relative energies of the states on regular and tilted lattices.

In all the calculations reported in this work, the DMRG solution of the impurity problem is

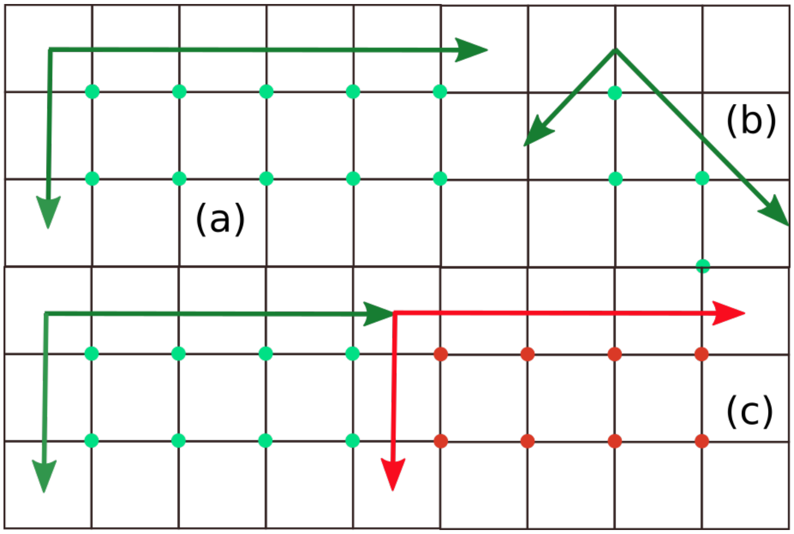


Figure S37: Impurity clusters used in the DMET calculations: (a) $\lambda \times 2$ clusters. (b) $\lambda\sqrt{2} \times \sqrt{2}$ clusters. (c) $\lambda \times 2$ clusters with time inversion on neighboring clusters. Additional data on $4 \times 4$ clusters is in Ref. (*19*).

converged in terms of truncation error, and the DMET uncertainty comes from the convergence of the correlation potential. We report the energy and its uncertainty as the average and half of the difference of the last two DMET cycles, respectively.

## S9.2 DMET results for U=8

The charge and spin orders of the vertical stripes are plotted in Fig. S38. The corresponding energies are displayed in Table S1. No pairing order is observed at any the wavelengths except for $\lambda = 9$. However, for $\lambda = 9$, the DMET cycles are significantly harder to converge, indicating frustration in the system. The calculation also results in a much higher energy than the $\lambda = 8$ calculation.

In addition to the results shown here, we start with random initial guesses for the correlation potential on a $5 \times 2$ cell, to test the robustness of the solutions. Out of eight different initial guesses, five of them converge to the solution shown in Fig. S38(c); for the other three initial guesses, two of them converge to a stripe with a pair density wave, but with a much higher

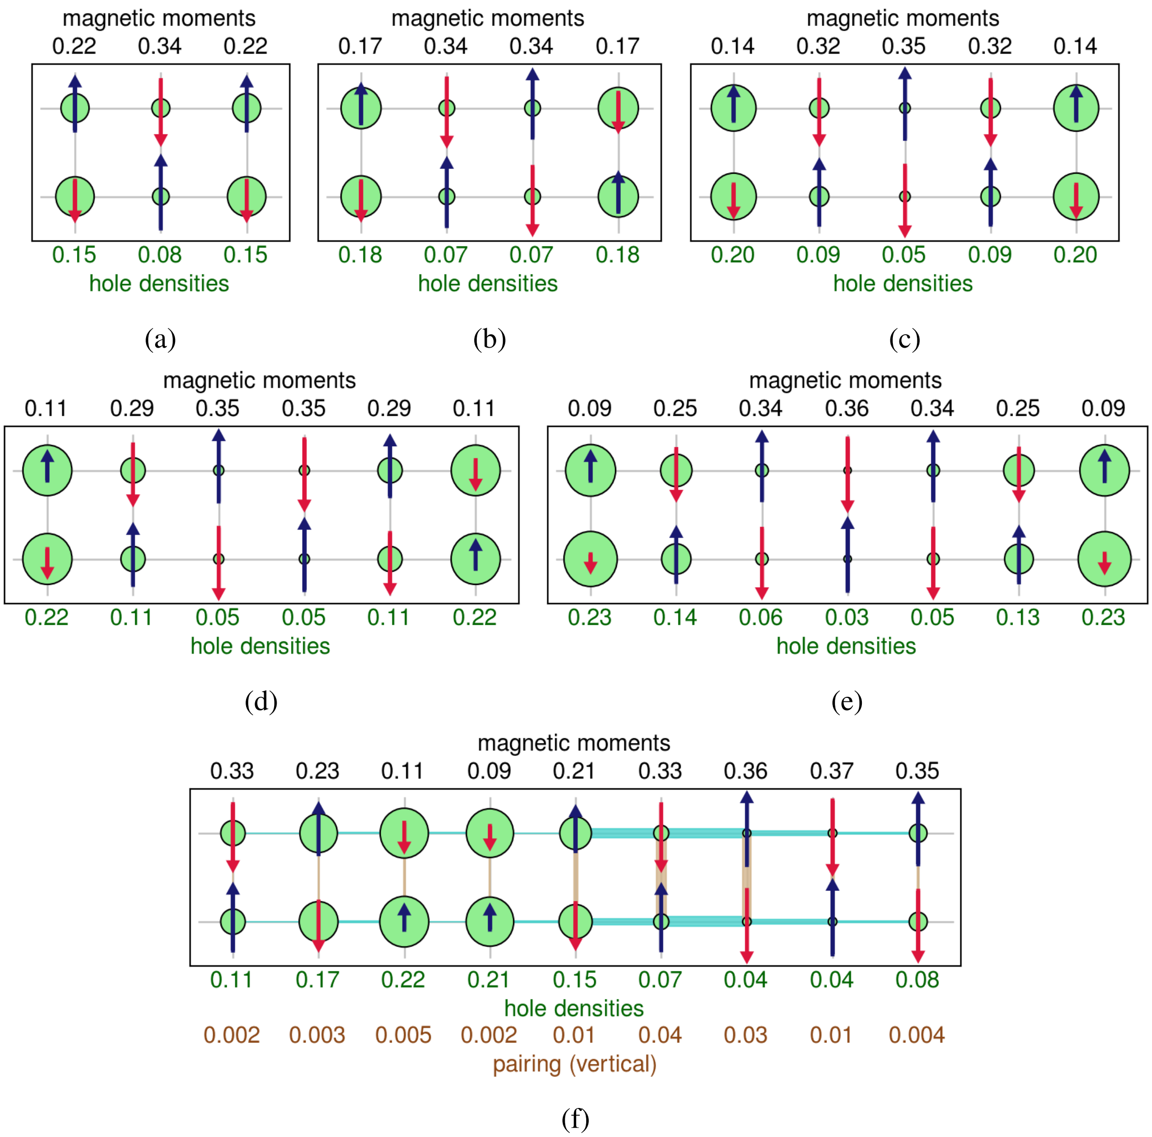


Figure S38: Spin and charge order of vertical stripes or stripe-like states from DMET calculations, for wavelength $3$, $4$, $5$, $6$, $7$ and $9$ at $U/t = 8$. The $\lambda = 8$ state is plotted in Fig. 4(a) in the main text. The spin is flipped between neighboring clusters for the even wavelength stripes.

energy (by $\sim 0.02t$ per site); one converges to a $d$-wave striped state, shown in Fig. 5 of the main text, with only a slightly higher energy ($\sim 0.003t$ per site).

We use tilted clusters to try to encourage diagonal stripes. Starting from different initial guesses, we obtain two stripe-like states in $5\sqrt{2} \times \sqrt{2}$ cluster calculations, shown in Fig. S39. To estimate the finite size correction, we use a $2\sqrt{2} \times \sqrt{2}$ cluster to compute the energy of the uniform $d$-wave state, obtaining $e = -0.76196(1)t$, compared to $e = -0.7580(4)t$ in a $2 \times 2$ regular cluster calculation. Computing a corrected energy of the diagonal striped state to compare to the vertical striped state as $E = E_{\sqrt{5}\times 2} - E_{\sqrt{2}\times 2} + E_{2\times 2}$, we find $\Delta e \sim 0.005t$ and $\Delta e \sim 0.036t$ for the two metastable diagonal stripe-like states, relative to the lowest energy vertical striped state.

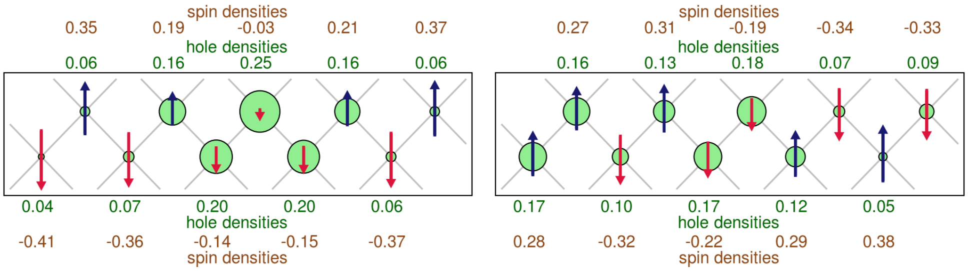


(a) $e = -0.769(1)$ (b) $e = -0.738(1)$

Figure S39: Spin and charge order of stripe-like states with wavevectors along the diagonal direction.

## S9.3 DMET results for U=6 and U=12

The DMET calculations are carried out for $U/t = 6$ and $U/t = 12$ as well. The methodology is the same as for $U/t = 8$. For even wavelengths, we carried out calculations on both regular periodic cells and spin-flipped cells, and used whichever gave the lower energy.

The patterns of stripes and other charge, spin and pairing orders for $U/t = 6$ and $U/t = 12$ are shown in Fig. S40 and Fig. S41, respectively.

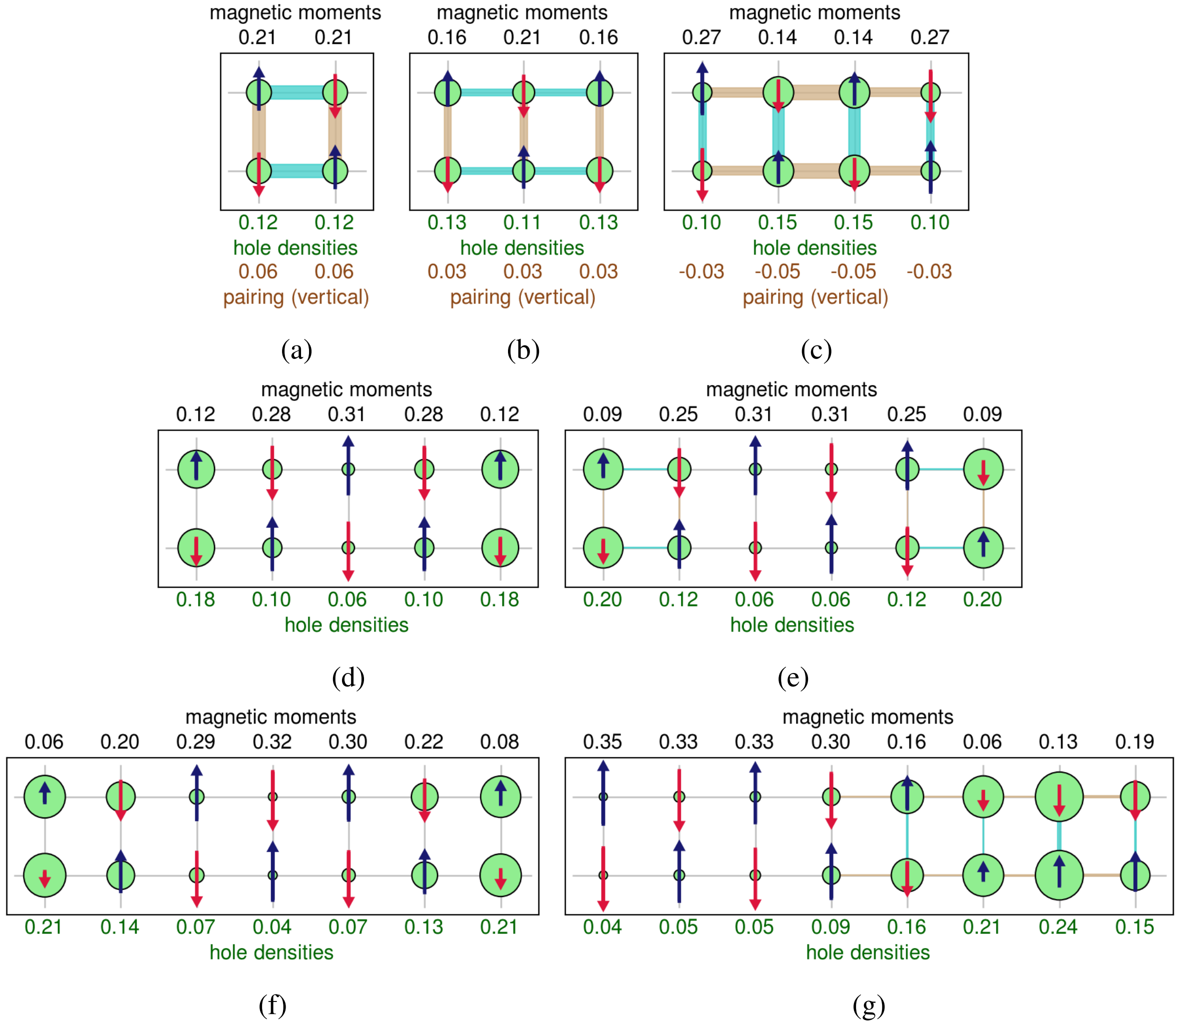


Figure S40: Spin and charge order of stripes, uniform $d$-wave states and spin density waves from DMET calculations, for plaquette and wavelength 3 to 8 at $U/t = 6$. The spin is flipped between neighboring clusters for the wavelength 6 and 8 stripes. Note that $\lambda = 4$ gives a spin density wave with $d$-wave pairing rather than a stripe.

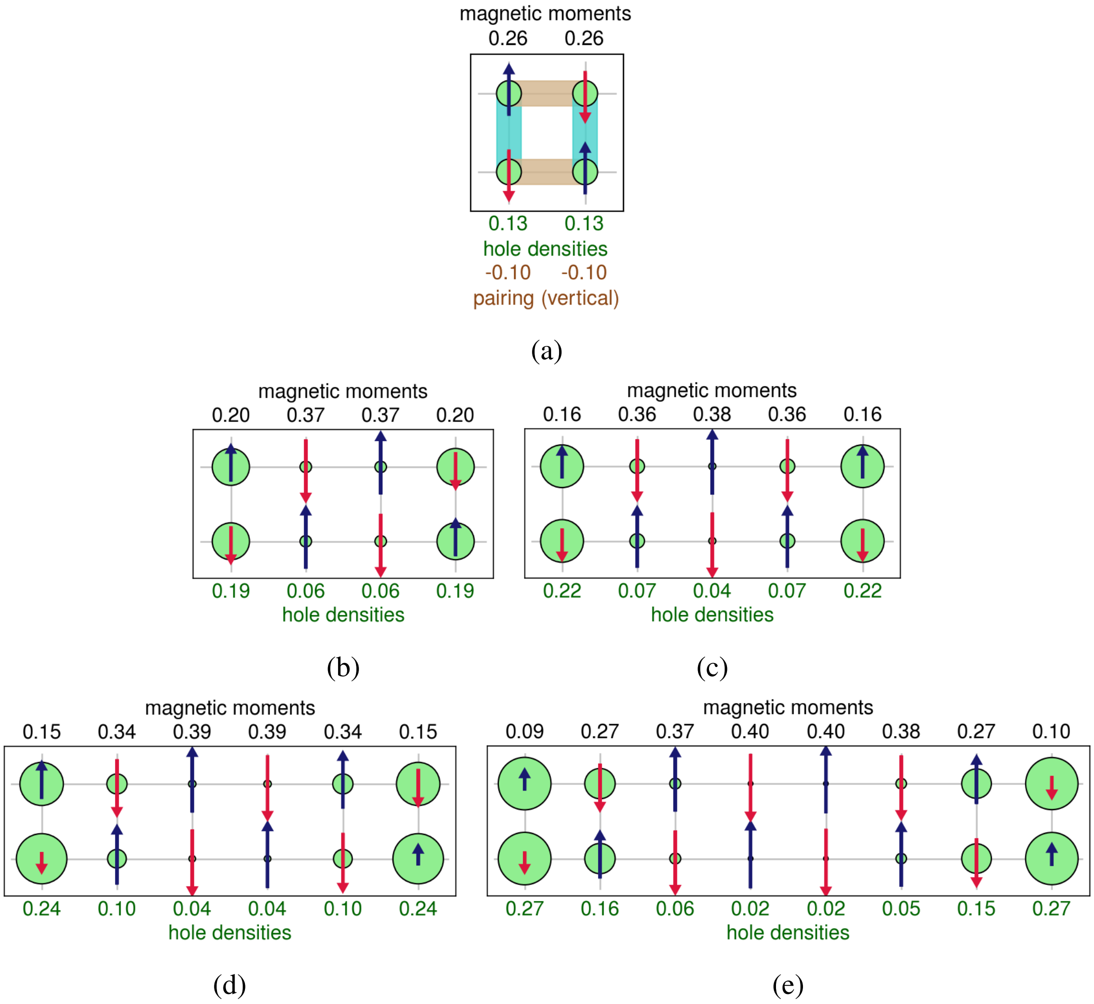


Figure S41: Spin and charge order of stripes and uniform $d$-wave states from DMET calculations, for plaquette and wavelength $4$, $5$, $6$ and $8$ at $U/t = 12$. The spin is flipped between neighboring clusters for the even-wavelength stripes.

# References


1. E. Dagotto, *Science* **309**, 257 (2005).
2. R. Comin, A. Damascelli, *Annual Reviews of Condensed Matter Physics* **7**, 369 (2016).
3. M.-H. Julien, *Science* **350**, 914 (2015).
4. C. V. Parker, *et al.*, *Nature* **468**, 677 (2010).
5. S. Gerber, *et al.*, *Science* **350**, 949 (2015).
6. E. Fradkin, S. A. Kivelson, J. M. Tranquada, *Reviews of Modern Physics* **87**, 457 (2015).
7. D. Poilblanc, T. M. Rice, *Phys. Rev. B* **39**, 9749 (1989).
8. J. Zaanen, O. Gunnarsson, *Physical Review B* **40**, 7391 (1989).
9. K. Machida, *Physica C: Superconductivity* **158**, 192 (1989).
10. H. Schulz, *Journal de Physique* **50**, 17 (1989).
11. V. Emery, S. Kivelson, H. Lin, *Physical review letters* **64**, 475 (1990).
12. V. J. Emery, S. Kivelson, H. Lin, *Physica B: Condensed Matter* **163**, 306 (1990).
13. S. R. White, D. J. Scalapino, *Phys. Rev. Lett.* **80**, 1272 (1998).
14. S. R. White, D. J. Scalapino, *Phys. Rev. Lett.* **91**, 136403 (2003).
15. G. Hager, G. Wellein, E. Jeckelmann, H. Fehske, *Physical Review B* **71**, 075108 (2005).
16. A. Himeda, T. Kato, M. Ogata, *Phys. Rev. Lett.* **88**, 117001 (2002).
17. C.-C. Chang, S. Zhang, *Physical review letters* **104**, 116402 (2010).

18. P. Corboz, T. Rice, M. Troyer, *Physical review letters* **113**, 046402 (2014).

19. B.-X. Zheng, G. K.-L. Chan, *Phys. Rev. B* **93**, 035126 (2016).

20. H. Yamase, A. Eberlein, W. Metzner, *Physical review letters* **116**, 096402 (2016).

21. S. Sorella, *et al.*, *Physical review letters* **88**, 117002 (2002).

22. W.-J. Hu, F. Becca, S. Sorella, *Phys. Rev. B* **85**, 081110 (2012).

23. A. Macridin, M. Jarrell, T. Maier, *Physical Review B* **74**, 085104 (2006).

24. J. P. F. LeBlanc, *et al.*, *Phys. Rev. X* **5**, 041041 (2015).

25. M. Raczkowski, M. Capello, D. Poilblanc, R. Frésard, A. M. Oles, *Phys. Rev. B* **76**, 140505 (2007).

26. C.-P. Chou, N. Fukushima, T. K. Lee, *Phys. Rev. B* **78**, 134530 (2008).

27. C.-P. Chou, T.-K. Lee, *Phys. Rev. B* **81**, 060503 (2010).

28. S. White, *et al.*, *Physical Review B* **40**, 506 (1989).

29. W. Wu, M. Ferrero, A. Georges, E. Kozik, *Physical Review B* **96**, 041105 (2017).

30. Supplementary information.

31. S. Zhang, J. Carlson, J. E. Gubernatis, *Phys. Rev. Lett.* **74**, 3652 (1995).

32. C.-C. Chang, S. Zhang, *Phys. Rev. B* **78**, 165101 (2008).

33. M. Qin, H. Shi, S. Zhang, *Physical Review B* **94**, 235119 (2016).

34. J. Motruk, M. P. Zaletel, R. S. K. Mong, F. Pollmann, *Phys. Rev. B* **93**, 155139 (2016).

35. E. Stoudenmire, S. R. White, *Annual Review of Condensed Matter Physics* **3**, 111 (2012).

36. G. Knizia, G. K.-L. Chan, *Physical review letters* **109**, 186404 (2012).

37. F. Verstraete, J. I. Cirac, *arXiv:cond-mat/0407066* (2004).

38. Y. Nishio, N. Maeshima, A. Gendiar, T. Nishino, *arXiv:cond-mat/0401115* (2004).

39. J. Jordan, R. Orús, G. Vidal, F. Verstraete, J. I. Cirac, *Physical review letters* **101**, 250602 (2008).

40. J. Tranquada, B. Sternlieb, J. Axe, Y. Nakamura, S. Uchida, *Nature* **375**, 561 (1995).

41. A. V. Chubukov, K. A. Musaelian, *Phys. Rev. B* **51**, 12605 (1995).

42. M. Vojta, *Physical Review B* **66**, 104505 (2002).

43. S. R. White, D. Scalapino, *Physical Review B* **70**, 220506 (2004).

44. M. Kato, K. Machida, H. Nakanishi, M. Fujita, *Journal of the Physical Society of Japan* **59**, 1047 (1990).

45. J. F. Dodaro, H.-C. Jiang, S. A. Kivelson, *Physical Review B* **95**, 155116 (2017).

46. J. Xu, S. Chiesa, E. J. Walter, S. Zhang, *Journal of Physics: Condensed Matter* **25**, 415602 (2013).

47. V. Emery, S. Kivelson, O. Zachar, *Physical Review B* **56**, 6120 (1997).

48. S. A. Kivelson, E. Fradkin, V. J. Emery, *Nature* **393**, 550 (1998).

49. J. Zaanen, O. Osman, H. Kruis, Z. Nussinov, J. Tworzydlo, *Philosophical Magazine B* **81**, 1485 (2001).

50. H.-B. Schüttler, C. Gröber, H. Evertz, W. Hanke, *arXiv:cond-mat/0104300* (2001).

51. E. Arrigoni, A. Harju, W. Hanke, B. Brendel, S. Kivelson, *Physical Review B* **65**, 134503 (2002).

52. We construct the trial wave-function with desired wave-length by solving the non-interacting Hamiltonian with pinning fields in the whole system with the same structure.

53. M. Qin, H. Shi, S. Zhang, *Phys. Rev. B* **94**, 085103 (2016).

54. F. Verstraete, V. Murg, J. I. Cirac, *Advances in Physics* **57**, 143 (2008).

55. T. Nishino, *et al.*, *Prog. Theor. Phys.* **105**, 409 (2001).

56. J. Eisert, M. Cramer, M. B. Plenio, *Rev. Mod. Phys.* **82**, 277 (2010).

57. P. Corboz, *Phys. Rev. B* **93**, 045116 (2016).

58. P. Corboz, R. Orus, B. Bauer, G. Vidal, *Phys. Rev. B* **81**, 165104 (2010).

59. H. N. Phien, J. A. Bengua, H. D. Tuan, P. Corboz, R. Orus, *Phys. Rev. B* **92**, 035142 (2015).

60. H. C. Jiang, Z. Y. Weng, D. N. Sheng, *Phys. Rev. Lett.* **101**, 117203 (2008).

61. P. Corboz, S. R. White, G. Vidal, M. Troyer, *Phys. Rev. B* **84**, 041108 (2011).

62. T. Nishino, K. Okunishi, *J. Phys. Soc. Jpn.* **65**, 891 (1996).

63. R. Orús, G. Vidal, *Phys. Rev. B* **80**, 094403 (2009).

64. S. Singh, R. N. C. Pfeifer, G. Vidal, *Phys. Rev. B* **83**, 115125 (2011).

65. B. Bauer, P. Corboz, R. Orús, M. Troyer, *Phys. Rev. B* **83**, 125106 (2011).

66. P. Corboz, G. Vidal, *Phys. Rev. B* **80**, 165129 (2009).

67. B.-X. Zheng, J. S. Kretchmer, H. Shi, S. Zhang, G. K.-L. Chan, *Physical Review B* **95**, 045103 (2017).
